# Supplementary material for: Scalable simulation-based inference for implicitly defined models using a metamodel for Monte Carlo log-likelihood estimator
Source: arXiv:2311.09446 source file (2025-04-16)
Supplement: Supplementary file 1 [file ms-supp_arxiv_v3.pdf]

# Supplementary text for *Scalable simulation-based inference for implicitly defined models using a metamodel for Monte Carlo log-likelihood estimator*

Joonha Park

Department of Mathematics, University of Kansas, Lawrence, KS 66045 USA
(email: j.park@ku.edu)

## S1 Further details on the simulation-based proxy $\mathcal{R}(\theta_0)$ and inference bias

### S1.1 Simulation-based proxy and MESLE for several iid examples

In this section, we compute the MESLE and the simulation-based proxy for several examples.

**Example S1.** Suppose that the latent process is given by $n$ iid copies of Gamma random variables $X_1, \dots, X_n \sim \Gamma(\gamma, \lambda)$ with shape parameter $\gamma$ and rate parameter $\lambda$. Partial observations $Y_1, \dots, Y_n$ are given by $Y_i | X_i \sim \text{Pois}(X_i)$. Since $X_i = G_i/\lambda$ for $G_i \sim \Gamma(\gamma, 1)$, the expected simulated log-likelihood at $\lambda$ is given by

$$\mu(\lambda; y_i) = \mathbb{E}\left[-X_i + y_i \log X_i + \text{const.}\right] = -\gamma\lambda^{-1} - y_i \log \lambda + \text{const.}$$

where the constant terms do not depend on $\lambda$. The expected simulated log-likelihood for $n$ observations $y_{1:n}$ is given by

$$\mu(\lambda; y_{1:n}) = -n\gamma\lambda^{-1} - \textstyle\sum_i y_i \cdot \log \lambda + \text{const.}$$

and the MESLE is given by $\lambda_{MESLE} = n\gamma / \sum_i y_i$. Each $Y_i$ marginally follows the negative binomial distribution with probability mass function

$$p_\lambda^Y(y) = \frac{\Gamma(y+\gamma)}{\Gamma(y+1)\Gamma(\gamma)} \left(\frac{1}{1+\lambda}\right)^y \left(\frac{\lambda}{1+\lambda}\right)^\gamma.$$

Thus it can be checked that MLE for $\lambda$ is equal to the MESLE for this model.

The data-averaged expected simulated log-likelihood for $n$ observations is given by

$$U(\lambda_0, \lambda) = \mathbb{E}_{Y_{1:n} \overset{iid}{\sim} P_{\lambda_0}^Y} \mu(\lambda; Y_{1:n}) = -n\gamma\lambda^{-1} - n\gamma\lambda_0^{-1} \log \lambda + \text{const.},$$

since the marginal mean of $Y$ is equal to $\gamma\lambda_0^{-1}$. The simulation-based proxy $\mathcal{R}(\lambda_0)$ is thus equal to $\lambda_0$.

The matrix $K_1(\lambda_0)$ is given by

$$K_1(\lambda_0) = \frac{1}{n}\text{Var}_{\lambda_0}\left[\frac{\partial \mu}{\partial \lambda}(\lambda_*; Y_{1:n})\right] = \frac{1}{n}\lambda_*^{-2}\text{Var}(\sum_i Y_i) = \lambda_*^{-2}\gamma(1+\lambda_0)\lambda_0^{-2} = \gamma\lambda_0^{-4}(1+\lambda_0).$$

The matrix $K_2(\lambda_0)$ is given by

$$K_2(\lambda_0) = -\frac{1}{n}\mathbb{E}\,\frac{\partial^2}{\partial\lambda^2}\mu(\lambda_*; Y_{1:n}) = -\mathbb{E}\left[-2\gamma\lambda_*^{-3} + (\sum_i Y_i)\lambda_*^{-2}\right] = 2\gamma\lambda_*^{-3} - \lambda_*^{-2} \cdot \gamma\lambda_0^{-1} = \gamma\lambda_0^{-3}.$$

Note that this $K_2(\lambda_0)$ differs from the Fisher information for the marginal distribution of $Y$, which is given by

$$\mathcal{I}(\lambda_0) = \gamma(1+\lambda_0)^{-1}\lambda_0^{-2}.$$

For the parameter values $\gamma = 1$ and $\lambda_0 = 1$ used in Section 5.1, $K_1(\lambda_0) = 2$, $K_2(\lambda_0) = 1$ and $\mathcal{I}(\lambda_0) = \frac{1}{2}$. Note that $K_1(\lambda_0)$ and $K_2(\lambda_0)$ are different. Additionally, the fact that $K_2(\lambda_0)$ differs from $\mathcal{I}(\lambda_0)$ aligns with the observation from Figure 2 that the second derivative of the estimated $\mu$ fuction (blue dashed curve) was greater in magnitude than that of the log-likelihood function (red dashed curve).

**Example S2.** Consider a normal model $X_1, \ldots, X_n \overset{iid}{\sim} \mathcal{N}(\theta, I_d)$ where $\theta \in \mathbb{R}^d$. Partial observations are given by $Y_i|X_i \sim \mathcal{N}(X_i, I_d)$. Marginally, we have $Y_i \sim \mathcal{N}(\theta, 2I_d)$. The expected simulated log-likelihood for $n$ observations $y_{1:n}$ is given by

$$\mu(\theta; y_{1:n}) = -\frac{1}{2}\sum_{i=1}^{n} \|y_i - \theta\|^2 + \text{const.} = -\frac{1}{2}\left(\sum_{i=1}^{n} \|y_i - \bar{y}\|^2 + n\|\bar{y} - \theta\|^2\right) + \text{const.}$$

where $\bar{y} := \frac{1}{n}\sum_{i=1}^{n} y_i$. The MESLE is given by $\theta_{MESLE} = \bar{y}$, which is equal to the MLE. The data-averaged expected simulated log-likelihood for $n$ observations is given by

$$U(\theta_0, \theta) = \mathbb{E}_{Y_{1:n} \overset{iid}{\sim} \mathcal{N}(\theta_0, 2I_d)}\, \mu(\theta; Y_{1:n}) = -\frac{n}{2}\|\theta - \theta_0\|^2 + \text{const.}$$

Therefore the simulation-based proxy $\mathcal{R}(\theta_0)$ is equal to $\theta_0$.

**Example S3.** Consider the normal model $X_1, \ldots, X_n \overset{iid}{\sim} \mathcal{N}(0, \Sigma)$ and $Y_i|X_i \sim \mathcal{N}(X_i, \Psi)$, where $\Psi$ is known and $\Sigma$ is the unknown parameter. The expected simulated log-likelihood is given by

$$\mu(\Sigma; y_{1:n}) = -\frac{1}{2}\left\{\sum_{i=1}^{n} y_i^\top \Psi^{-1} y_i + n\text{Tr}(\Psi^{-1}\Sigma)\right\} - \frac{n}{2}\log\det\Psi + \text{const.}$$

Therefore the MESLE is given by $\Sigma_{MESLE} = 0$. However, the MLE is given by $\Sigma_{MLE} = \frac{1}{n}\sum_i y_i y_i^\top - \Psi$. It can be seen that the simulation-based proxy $\mathcal{R}(\Sigma_0)$ is the zero matrix, thus again different from the true value $\Sigma_0$.

**Example S4.** Consider the same model $X_1, \ldots, X_n \overset{iid}{\sim} \mathcal{N}(0, \Sigma)$ and $Y_i|X_i \sim \mathcal{N}(X_i, \Psi)$ as in Example S3, but suppose that $\Sigma$ is known and $\Psi$ is the unknown parameter. It can be checked that the MESLE is given by $\Psi_{MESLE} = \frac{1}{n}\sum_i y_i y_i^\top + \Sigma$. However, the MLE for $\Psi$ is given by $\hat{\Psi}_{\text{MLE}} = \frac{1}{n}\sum_{i=1}^{n} y_i y_i^\top - \Sigma$. The data-averaged expected simulated log-likelihood is given by

$$U(\Psi_0, \Psi) = -\frac{n}{2}\text{Tr}\{\Psi^{-1}(2\Sigma + \Psi_0)\} - \frac{n}{2}\log\det\Psi + \text{const.},$$

and the simulation-based proxy is given by $\mathcal{R}(\Psi_0) = 2\Sigma + \Psi_0$. Thus both the MESLE and the simulation-based proxy have a bias of $2\Sigma$.

## S1.2 Simulation-based proxy from an information theoretic perspective

In the case where the simulated log-likelihood is given by $\log g(y|X;\theta)$, the simulation-based proxy $\mathcal{R}(\theta_0)$ may be interpreted from an information-theoretic perspective as follows (see Proposition S1). The KL divergence between two distributions $P$ and $Q$ with densities $p$ and $q$, respectively, will be denoted by

$$D_{KL}(P||Q) = \int \log\frac{\mathrm{d}P}{\mathrm{d}Q}\,\mathrm{d}P = D_{KL}(p||q) = \int \log\frac{p(y)}{q(y)}p(y)\,\mathrm{d}y.$$

In our parameterized setting we define the expected Kullback-Leibler divergence between $P_{\theta_0}$ and $P_\theta$ as

$$EKL(\theta_0||\theta) := \int D_{KL}(g_{x',\theta_0}||g_{x,\theta})\,\mathrm{d}P_{\theta_0}(x')\,\mathrm{d}P_\theta(x),$$

where we write $g_{x,\theta}(y) \equiv g(y|x;\theta)$. The simulation-based proxy minimizes the expected KL divergence between $P_{\theta_0}^Y$ and $g_{X,\theta}$ as well as that between $g_{X',\theta_0}$ and $g_{X,\theta}$ where $X' \sim P_{\theta_0}$ is independent of $X \sim P_\theta$.

**Proposition S1.** *If the simulated log-likelihood $\ell^S(\theta; y)$ is given by $\log g(y|X;\theta)$ where $X$ is a draw from $P_\theta$, the simulation-based proxy satisfies*

$$\mathcal{R}(\theta_0) = \underset{\theta\in\Theta}{\arg\min}\, \mathbb{E}_{X\sim P_\theta}\, D_{KL}(p^Y_{\theta_0}||g_{X,\theta}) = \underset{\theta\in\Theta}{\arg\min}\, EKL(\theta_0||\theta).$$

*Proof of Proposition S1.* This follows from Proposition S1, because the first terms in (S1) and (S2) do not depend on $\theta$. □

**Lemma S1.** *Let the Shannon entropy of a density $p$ be given by $H(p) = -\int \log p(y)\cdot p(y)\,\mathrm{d}y$. If the simulated log-likelihood $\ell^S(\theta; y)$ is given by $\log g(y|X,\theta)$ where $X$ is a draw from $P_\theta$, the data-averaged simulated log-likelihood satisfies*

$$U(\theta_0,\theta) = -H(p^Y_{\theta_0}) - \mathbb{E}_{X\sim P_\theta}\, D_{KL}(p^Y_{\theta_0}||g_{X,\theta}) \tag{S1}$$

$$= -\mathbb{E}_{X\sim P_{\theta_0}}\, H(g_{X,\theta_0}) - EKL(\theta_0||\theta) \tag{S2}$$

*Proof of Lemma S1.*

$$\begin{aligned} U(\theta_0,\theta) &= \int \log g_{x,\theta}(y)\,\mathrm{d}P_\theta(x)\,\mathrm{d}P^Y_{\theta_0}(y) \\ &= \int \left[\log p^Y_{\theta_0}(y) - \log \frac{p^Y_{\theta_0}(y)}{g_{x,\theta}(y)}\right] \mathrm{d}P_\theta(x)\,\mathrm{d}P^Y_{\theta_0}(y) \\ &= -H(p^Y_{\theta_0}) - \mathbb{E}_{X\sim P_\theta}\, D_{KL}(p^Y_{\theta_0}||g_{X,\theta}). \end{aligned}$$

On the other hand,

$$\begin{aligned} \int \log g_{x,\theta}(y)\cdot g_{x',\theta_0}(y)\,\mathrm{d}y &= -\int \log \frac{g_{x',\theta_0}(y)}{g_{x,\theta}(y)} g_{x',\theta_0}(y)\,\mathrm{d}y + \int \log g_{x',\theta_0}(y)\cdot g_{x',\theta_0}(y)\,\mathrm{d}y \\ &= -D_{KL}(g_{x',\theta_0}||g_{x,\theta}) - H(g_{x',\theta_0}). \end{aligned}$$

Integrating the above display with respect to $dP_{\theta_0}(x')\,dP_\theta(x)$, we obtain (S2). □

# S2 Further mathematical details on Section 2

## S2.1 Sufficient conditions for Assumption 3 for marginally dependent $Y_{1:n}$

If $Y_{1:n}$ are marginally independent, then Assumption 3 is satisfied under suitable conditions on the moments by the Lindeberg-Feller central limit theorem [5]. Here we consider some cases where $Y_{1:n}$ are marginally dependent but where Assumption 3 is still satisfied.

**Example S5.** Let $X = \{X_i; 1 \le i \le n\}$ be a $k$-dependent stochastic process for some $k \ge 1$, meaning that the $\sigma$-algebra $\mathcal{F}_i = \sigma(X_j; j \le i)$ is independent of $\mathcal{F}'_{i+k} = \sigma(X_j; j > i+k)$ for all $i$. Let $Y = \{Y_i; 1 \le i \le n\}$ be a collection of *local* observations of $X$. That is, $Y_i$ depends only on $\{X_j; j \in \mathcal{N}(i)\}$ where $\mathcal{N}(i) \subseteq \{\max(i-b,1),\ldots,\min(i+b,n)\}$ for some fixed $b \ge 1$, such that $g_i(Y_i|X) = g_i(Y_i|X_{\mathcal{N}(i)})$. Then $Y_i$ and $Y_{i+2b+k+1}$ are independent, since $X_{\mathcal{N}(i)} \in \mathcal{F}_{i+b}$ and $X_{\mathcal{N}(i+2b+k+1)} \in \mathcal{F}'_{i+b+k}$ are independent. It follows that the sequence $\{\frac{\partial\mu_i}{\partial\theta}(\theta_*; Y_i); i \ge 1\}$ is $2b+k$-dependent. If $\{\frac{\partial\mu_i}{\partial\theta}(\theta_*; Y_i); i \ge 1\}$ are uniformly bounded and satisfy $\mathrm{Var}\{\sum_{i=1}^n \frac{\partial\mu_i}{\partial\theta}(\theta_*; Y_i)\}/n^{2/3} \to \infty$ as $n \to \infty$, the central limit theorem holds for the sequence $\{\frac{\partial\mu_i}{\partial\theta}(\theta_*; Y_i); i \ge 1\}$ by Chung [5, Theorem 7.3.1].

**Example S6.** Suppose that $X = \{X_i; i \ge 1\}$ is a strictly stationary and strongly mixing process. A process is strongly mixing if the strong mixing coefficient

$$\alpha_k := \sup\{|\mathsf{P}(A\cap B) - \mathsf{P}(A)\mathsf{P}(B)|; A \in \mathcal{F}_i, B \in \mathcal{F}'_{i+k-1}\}$$

converges to zero as $k \to \infty$. If the observations $Y_i$ are local in the sense described in Example S5 and $X$ is strongly mixing, then the sequence $\{\frac{\partial \mu_i}{\partial \theta}(\theta_*; Y_i); i \geq 1\}$ is also strongly mixing. Suppose that the sequence $\{\frac{\partial \mu_i}{\partial \theta}(\theta_*; Y_i); i \geq 1\}$ is strictly stationary and satisfies

$$\int_0^1 \alpha^{-1}(u) Q(u)^2 \, \mathrm{d}u < \infty \tag{S3}$$

where $\alpha^{-1}(u) = \inf\{k; \alpha_k \leq u\}$ and $Q(u) = \inf\{t; \mathsf{P}[\|\frac{\partial \mu_1}{\partial \theta}(\theta_*; Y_1)\| > t] \leq u\}$. Then according to Doukhan et al. [6, Theorem 1], the central limit theorem holds for the sequence $\{\frac{\partial \mu_i}{\partial \theta}(\theta_*; Y_i); i \geq 1\}$. For the special case where this sequence is $k$-dependent for some $k \geq 1$, the condition (S3) reduces to $\mathbb{E}\left\|\frac{\partial \mu_i}{\partial \theta}(\theta_*; Y_i)\right\|^2 < \infty$.

We note that the mixing conditions for $X$ mentioned in Examples S5 and S6 can also be used to justify the asymptotic normality of simulated log-likelihoods $\ell^S(\theta; y_{1:n})$ for a given set of observations $y_{1:n}$ (Assumption 6). Specifically, if the individual simulated log-likelihoods $\ell_i^S(\theta; y_i)$ depend locally on the simulated draw $X$ in the sense described in Example S5, then the central limit theorem applies to $\ell^S(\theta; y_{1:n})$ provided that $\ell_i^S(\theta; y_i)$ satisfy the same conditions on $\frac{\partial \mu_i}{\partial \theta}(\theta_*; Y_i)$ stated in Examples S5 or S6.

## S2.2 Proofs for Section 2.2

*Proof of Proposition 1.* Using Taylor's expansion with an integral remainder term, for $f : \mathbb{R} \to \mathbb{R}$ that is three times continuously differentiable at $a$, we have

$$f(x) = f(a) + f'(a)(x-a) + \frac{1}{2} f''(a)(x-a)^2 + \int_a^x f'''(t) \frac{(x-t)^2}{2} \, \mathrm{d}t. \tag{S4}$$

Consider a bounded set $B$ containing zero. Applying this result to three times differentiable function $\tau \mapsto \mu_i(\theta_* + \tau \frac{t}{\sqrt{n}})$ where $t \in B$, we obtain

$$\begin{aligned}\mu_i(\theta_* + \frac{t}{\sqrt{n}}; Y_i) = \mu_i(\theta_*; Y_i) + \frac{\partial \mu_i}{\partial \theta}(\theta_*; Y_i) \frac{t}{\sqrt{n}} + \frac{1}{2n} t^\top \frac{\partial^2 \mu_i}{\partial \theta^2}(\theta_*; Y_i) t \\ + \frac{1}{2n^{3/2}} \int_0^1 \frac{\partial^3 \mu_i}{\partial \theta^3}(\theta_* + \tau \frac{t}{\sqrt{n}}; Y_i)(t,t,t)(1-\tau)^2 \, \mathrm{d}\tau\end{aligned}$$

where $\frac{\partial^3 \mu_i}{\partial \theta^3}(\theta_*; Y_i) : \mathbb{R}^{3d} \to \mathbb{R}$ is a trilinear form given by

$$\frac{\partial^3 \mu_i}{\partial \theta^3}(\theta_*; Y_i)(t,s,r) = \sum_{k_1,k_2,k_3 \in 1:d} \frac{\partial^3 \mu_i}{\partial \theta_{(k_1)} \partial \theta_{(k_2)} \partial \theta_{(k_3)}}(\theta_*; Y_i) t_{k_1} s_{k_2} r_{k_3}, \quad \forall t,s,r \in \mathbb{R}^d.$$

By Assumption 3,

$$S_n = \frac{1}{\sqrt{n}} \sum_{i=1}^n \frac{\partial \mu_i}{\partial \theta}(\theta_*; Y_i)$$

converges in distribution to $\mathcal{N}(0, K_1(\theta_0))$, and by Assumption 4,

$$\frac{1}{n} \sum_{i=1}^n \frac{\partial^2 \mu_i}{\partial \theta^2}(\theta_*; Y_i)$$

converges in probability to $-K_2(\theta_0)$. The absolute value of the integral remainder term is bounded by

$$\begin{aligned}&\left| \int_0^1 \frac{\partial^3 \mu_i}{\partial \theta^3}(\theta_* + \tau \frac{t}{\sqrt{n}}; Y_i)(t,t,t)(1-\tau)^2 \, \mathrm{d}\tau \right| \\ &\qquad \leq \sup_{\tau \in [0,1]} \max_{k_1,k_2,k_3 \in 1:d} \left\| \frac{\partial^3 \mu_i}{\partial \theta_{(k_1)} \partial \theta_{(k_2)} \partial \theta_{(k_3)}}(\theta_* + \tau \frac{t}{\sqrt{n}}; Y_i) \right\| d^3 \|t\|_\infty^3 \int_0^1 (1-\tau)^2 \, \mathrm{d}\tau.\end{aligned}$$

For sufficiently large $n$, $\{\theta_* + \tau\frac{t}{\sqrt{n}}; t \in B, \tau \in [0,1]\}$ is contained in $B_0$ defined in Assumption 5. Therefore, we have

$$\sum_{i=1}^{n}\left[\mu_i(\theta_* + \frac{t}{\sqrt{n}}; Y_i) - \mu_i(\theta_*; Y_i)\right] = S_n^\top t - \frac{1}{2}t^\top K_2(\theta_0)t + R_n(t) + o_p(1)$$

where $o_p(1)$ signifies a term that is independent of $t$ and converges in probability to zero and where the remainder term $R_n(t)$ satisfies

$$\mathbb{E}\sup_{t\in B}|R_n(t)| \leq \frac{1}{6n^{1/2}}Cd^3\|t\|_\infty^3.$$

Thus by Markov's inequality, $R_n(t)$ converges in probability to zero uniformly for $t \in B$. □

# S3 Further details on Section 2.5 Bias in simulation-based inference

The simulation-based inference procedure outlined in Section 2 and developed in detail in Sections 3–4 may have a bias in general due to the use of a metamodel for the log-likelihood estimator. In this section, we examine the bias and develop bounds on the inference bias under certain conditions.

## S3.1 Power series expression for Jensen bias using the cumulants of simulated log-likelihood

We refer to the difference $B(\theta) = \ell(\theta) - \mu(\theta)$ as the Jensen bias, which is always nonnegative when the simulated log-likelihood is given by the log of an unbiased likelihood estimator. For hidden Markov models, an unbiased simulation likelihood can be obtained by running the bootstrap particle filter, as described by Algorithm 2. Berard et al. [4] showed that under certain conditions, the logarithm of this estimator, which we denote by $\ell^S(\theta)$, approximately follows

$$\ell^S(\theta) \approx \mathcal{N}\left(\ell(\theta) - \frac{1}{2}\sigma^2(\theta), \sigma^2(\theta)\right)$$

(see (11)). In this case, the Jensen bias can be approximated by half the variance in the simulated log-likelihood.

More generally, we will consider the situation where the simulation likelihood $e^{\ell^S(\theta)}$ is unbiased for the likelihood $L(\theta)$. This happens in all examples we consider in this paper, whether $\ell^S(\theta)$ is given by the log-measurement density $g_{1:n}(y_{1:n}|X)$ or by the log-likelihood estimate produced by the bootstrap particle filter. Provided that the simulation likelihood is unbiased for the likelihood, the log-likelihood can be expressed as

$$\ell(\theta) = \log \mathbb{E}\, e^{\ell^S(\theta)}. \tag{S5}$$

The cumulant generating function, or the second characteristic function, $\psi(z)$ of a random variable $X$ is defined as the principal branch of the logarithm of its characteristic function [9, 11],

$$\psi(z) := \log \mathbb{E}\, e^{izX}.$$

The cumulant generating function is uniquely continuously defined on real intervals containing zero on which $\phi_X(s)$ is nonzero. If we denote by $\psi(z)$ the cumulant generating function for the simulated log-likelihood $\ell^S(\theta)$, we may express $\ell(\theta)$ as

$$\ell(\theta) = \log \mathbb{E}\, e^{\ell^S(\theta)} = \psi(-i), \tag{S6}$$

provided that $\psi(z)$ can be extended to a complex domain $|z| < R$ for some $R > 1$. Conditions under which an analytic extension of $\psi(z)$ is possible is discussed below. Under those conditions, $\psi(z)$ can be expressed as an absolutely convergent power series,

$$\psi(z) = \sum_{n=1}^{\infty}\frac{i^n\kappa_n(\theta)}{n!}z^n, \qquad |z| < R. \tag{S7}$$

The number $\kappa_n(\theta)$ is the $n$-th order cumulant of $\ell^S(\theta)$. The first two cumulants corresponding to $n = 1, 2$ are equal to the mean and the variance of the random variable. The log-likelihood $\ell(\theta)$ can thus be expressed as

$$\ell(\theta) = \sum_{j=1}^{\infty} \frac{\kappa_j(\theta)}{j!}. \tag{S8}$$

The expected simulated log-likelihood $\mu(\theta)$ can be considered as a first order approximation to (S8), since $\mu(\theta) = \kappa_1(\theta)$. The Jensen bias is given by

$$B(\theta) = \ell(\theta) - \mu(\theta) = \sum_{j \geq 2} \frac{\kappa_j(\theta)}{j!}. \tag{S9}$$

In the special case where $\ell^S(\theta)$ exactly follows the normal distribution with mean $\mu(\theta)$ and variance $\sigma^2(\theta)$, the analytic characteristic function is given by $\exp(i\mu(\theta)z - \frac{\sigma^2(\theta)z^2}{2})$, which is nowhere equal to zero. Thus the cumulant generating function is defined and analytic on the entire complex plane, and the log-likelihood is given by

$$\ell(\theta) = \psi(-i; \theta) = \kappa_1(\theta) + \frac{\kappa_2(\theta)}{2} = \mu(\theta) + \frac{\sigma^2(\theta)}{2}. \tag{S10}$$

The Jensen bias is equal to $B(\theta) = \sigma^2(\theta)/2$. We note, however, that even when the centered and scaled simulated log-likelihood $\frac{\ell^S(\theta; y_{1:n}) - \mu(\theta; y_{1:n})}{\sigma(\theta; y_{1:n})}$ converges to the normal distribution as $n \to \infty$ (Assumption 6), the higher order terms ($j \geq 3$) in (S9) do not approach zero in general. For instance, if the simulated log-likelihoods for the observation pieces $\{\ell^S(\theta; y_i); i \in 1:n\}$ are independent of each other, we have

$$\ell(\theta; y_{1:n}) = \log \mathbb{E}\, e^{\sum_{i=1}^n \ell^S(\theta; y_i)} = \sum_{i=1}^{n} \log \mathbb{E}\, e^{\ell^S(\theta; y_i)} = \sum_{j \geq 1} \frac{\sum_{i=1}^n \kappa_j(\theta; y_i)}{j!},$$

and thus all cumulants $\kappa_j(\theta; y_{1:n})$, $j \geq 1$, scale linearly with $n$.

We will now discuss the conditions for analytic extensions of the characteristic function and the cumulant generating function. A characteristic function $\phi(s)$ is called an analytic characteristic function if there is an analytic function on a complex circle $|z| < \rho$ (where $\rho > 0$) that agrees with $\phi(s)$ on some real neighborhood of zero, say $(-\epsilon, \epsilon)$ [11]. The extended function defined on a complex domain will also be called the analytic characteristic function and denoted by $\phi(z)$. The extended analytic characteristic function has a Maclaurin series expansion about zero.

**Theorem S1.** *Suppose that a random variable with cumulative distribution function (cdf) $F$ has an analytic characteristic function $\phi(z)$. The Maclaurin series of the analytic characteristic function*

$$\phi(z) = \sum_{n=0}^{\infty} \frac{i^n \alpha_n}{n!} z^n \tag{S11}$$

*is absolutely convergent on a complex disk $|z| < R$ for some positive $R$ if and only if the relation*

$$1 - F(x) + F(-x) = o(e^{-rx}) \quad \text{as} \quad x \to \infty$$

*holds for all positive $r < R$. Then the $n$-th moment of the random variable is given by $\alpha_n = i^{-n}\phi^{(n)}(0)$, where $\phi^{(n)}$ denotes the $n$-th derivative of $\phi$.*

*Proof.* This follows from Theorem 7.1.1, Corollary to Theorem 7.1.1, and Theorem 7.2.1 of Lukacs [11] and Chapter 5, Theorem 3 of Ahlfors [3]. □

Theorem S1 implies that the Maclaurin series (S11) for $\phi(z)$ converges at $z = -i$ if both $1 - F(x)$ and $F(-x)$ decays faster than $e^{-rx}$ as $x \to \infty$ for all $r < R$ for some $R > 1$. The first condition that $1 - F(x)$ decays faster than $e^{-rx}$ is almost satisfied if the likelihood $L(\theta)$ is finite. If we denote the cumulative distribution function of $\ell^S(\theta)$ by $F$, we have

$$\infty > L(\theta) = \mathbb{E}\, e^{\ell^S(\theta)} = \int_{-\infty}^{\infty} e^x \, \mathrm{d}F(x) \geq e^c(1 - F(c)) \quad \text{for all } c.$$

Therefore, $1 - F(x) = o(-rx)$ for all $r < 1$. However, this result is weaker than the required condition that $1 - F(x) = o(e^{-rx})$ for all $r < R$ for some $R > 1$.

The condition regarding the other tail, $F(-x) = o(e^{-rx})$ for $r < R$, can be readily satisfied if we truncate the simulated log-likelihood $\ell^S(\theta)$ from below, say at $-C$ for some large $C$. If $\ell^S(\theta) \geq -C_0$ with probability at least $p$ for some $C_0$, then we have

$$\begin{aligned}\log \mathbb{E}\, e^{\max(\ell^S, -C)} - \ell &\leq \log \frac{\mathbb{E}\, e^{\ell^S} 1[\ell^S \geq -C] + e^{-C}\mathsf{P}[\ell^S < -C]}{\mathbb{E}\, e^{\ell^S} 1[\ell^S \geq -C]} \\ &\leq \frac{e^{-C}\mathsf{P}[\ell^S < -C]}{\mathbb{E}\, e^{\ell^S} 1[\ell^S \geq -C]} \leq \frac{e^{-C}}{pe^{-C_0}} = p^{-1}e^{C_0 - C},\end{aligned}$$

and this truncation error can be bounded by an arbitrarily small number by taking $C$ sufficiently large.

If the analytic extension of the characteristic function $\phi(z)$ is nonzero anywhere in a disk $|z| < R$, then the cumulant generating function can be extended analytically to the same complex disk. For an analytic, nonzero function on $|z| < R$, an analytic, single-branched logarithm can be defined in that disk (see e.g., Chapter 4, Corollary to Theorem 16 in Ahlfors [3].) Here, that the logarithm is single-branched means that its value at any given point $z$ is defined as a single number, not up to integer multiples of $2\pi i$. We define an extended cumulative generating function $\psi(z)$ on the complex disk $|z| < R$ as the single-branched logarithm of $\phi(z)$ which is equal to zero at $z = 0$. Since this $\psi(z)$ is analytic on $|z| < R$, an absolutely convergent power series expansion of $\psi(z)$ about $z = 0$ is available, giving (S7).

We note that the preceding analysis suggests consideration of a higher order MESLE and a higher order simulation-based proxy defined as follows.

**Definition S1.** Let $\kappa_j(\theta; y_{1:n})$ be the $j$-th order cumulant of the simulated log-likelihood $\ell^S(\theta; y_{1:n})$ for $j \geq 1$. The $k$-th order maximum expected simulated log-likelihood (MESLE) for $k \geq 1$ is defined as

$$\hat{\theta}_{[k]}(y_{1:n}) := \arg\max_\theta \sum_{j=1}^k \frac{\kappa_j(\theta; y_{1:n})}{j!}.$$

The $k$-th order simulation-based proxy ($k \geq 1$) is defined as

$$\mathcal{R}_{[k]}(\theta_0) := \arg\max_\theta \mathbb{E}_{Y_{1:n} \sim P^Y_{\theta_0}} \sum_{j=1}^k \frac{\kappa_j(\theta; Y_{1:n})}{j!}.$$

However, the practical utility of an higher-order MESLE is likely limited, because its estimator will involve high Monte Carlo variation.

## S3.2 Bound on the Jensen bias $\ell(\theta; y) - \mu(\theta; y)$

The Jensen bias $B(\theta)$ can be upper bounded in the case where the simulated log-likelihood $\ell^S(\theta)$ has a sub-Gaussian tail.

**Proposition S2.** *Suppose that for some $C, C' > 0$,*

$$\mathsf{P}[\ell^S(\theta) - \mu(\theta) \geq t] \leq \frac{C'}{\sqrt{2\pi}C} e^{-\frac{t^2}{2C^2}}$$

*for all $t \geq 0$. Then the Jensen bias satisfies*

$$B(\theta) \leq \frac{C^2}{2} + \log(1 + C').$$

*Proof of Proposition S2.* We use the following result: for any random variable $X$ with cumulative distribution function $F$,

$$\mathbb{E}\, e^X \leq 1 + \int_0^\infty e^t (1 - F(t))\, \mathrm{d}t. \tag{S12}$$

This is because

$$\begin{aligned}
\mathbb{E}\, e^X &= \mathbb{E}\, e^X \mathbf{1}[X < 0] + \mathbb{E}\, e^X \mathbf{1}[X \geq 0] \\
&\leq \mathsf{P}[X < 0] + \mathsf{P}[X \geq 0] + \int_0^\infty (e^x - 1) F(\mathrm{d}x) \\
&= 1 + \int_0^\infty \int_0^\infty e^t \mathbf{1}[t < x]\, \mathrm{d}t F(\mathrm{d}t) \\
&= 1 + \int_0^\infty e^t \int_0^\infty \mathbf{1}[x > t] F(\mathrm{d}x)\, \mathrm{d}t \\
&= 1 + \int_0^\infty e^t (1 - F(t))\, \mathrm{d}t.
\end{aligned}$$

Using (S12) for $X = \ell^S(\theta)$, we have

$$\begin{aligned}
\mathbb{E}\, e^{\ell^S(\theta)} &\leq 1 + \int_0^\infty e^t \frac{C'}{\sqrt{2\pi} C} e^{-\frac{t^2}{2C^2}}\, \mathrm{d}t \\
&= 1 + \int_0^\infty \frac{C'}{\sqrt{2\pi} C} e^{-\frac{1}{2C^2}(t - C^2)^2} e^{\frac{C^2}{2}}\, \mathrm{d}t \\
&\leq 1 + C' e^{\frac{C^2}{2}}.
\end{aligned}$$

Therefore, it follows that

$$\ell(\theta) = \log \mathbb{E}\, e^{\ell^S(\theta)} \leq \log(1 + C' e^{\frac{C^2}{2}}) \leq \log(e^{\frac{C^2}{2}} + C' e^{\frac{C^2}{2}}) = \frac{C^2}{2} + \log(1 + C').$$

□

We also have the following result. If the simulated log-likelihood for the $i$-th observation, $\ell_i^S(\theta; y_i)$, is almost surely at most $s_i(\theta)$ higher than $\mathbb{E}\, \ell_i^S(\theta)$, then the Jensen bias is upper bounded by $\sum_i s_i(\theta)$. This condition is satisfied, when the individual simulated log-likelihoods $\ell_i^S(\theta; y_i)$ are both upper and lower bounded, which may happen when the observation space is compact.

**Proposition S3.** *Suppose that $\ell_i^S(\theta; y_i) - \mu_i(\theta; y_i)$ is almost surely upper bounded by $s_i(\theta)$ for each $i \in 1\!:\!n$. Then we have*

$$B(\theta) \leq \sum_{i=1}^n s_i(\theta).$$

*Proof of Proposition S3.*

$$\ell(\theta) - \mu(\theta) = \log \mathbb{E}\, e^{\sum_i \{\ell^S(\theta; y_i) - \mu_i(\theta; y_i)\}} \leq \mathbb{E}\, e^{\sum_i s_i} = \sum_i s_i.$$

□

## S3.3 Bound on the inference bias $\mathcal{R}(\theta_0) - \theta_0$

In the current section, we will construct a bound on the difference between $\theta_0$ and $\mathcal{R}(\theta_0)$ using the upper bound on the Jensen bias developed in Section S3.1.

If the observations $Y_{1:n}$ are obtained under $\theta_0$, then the data-averaged log-likelihood $\mathbb{E}_{Y_{1:n} \sim P_{\theta_0}^Y} \ell(\theta; Y_{1:n})$ equals the negative cross entropy, denoted by $-H(\theta_0, \theta)$:

$$\mathbb{E}_{Y_{1:n} \sim P_{\theta_0}^Y} \ell(\theta; Y_{1:n}) = \int \{\log p_{\theta,n}^Y(y_{1:n})\} p_{\theta_0}^Y(y_{1:n})\, \mathrm{d}y_{1:n} =: -H(\theta_0, \theta).$$

We write $H(\theta_0, \theta_0) = H(\theta_0)$. The cross entropy $H(\theta_0, \theta)$ is minimized at $\theta = \theta_0$, because it is equal to $H(\theta_0) + D_{KL}(\theta_0 || \theta)$, where the Kullback-Leibler divergence $D_{KL}(\theta_0 || \theta)$ is minimized at $\theta = \theta_0$ [12].

On the other hand, by Definition 2, the data-averaged expected simulated log-likelihood $U(\theta_0, \theta)$ is maximized when $\theta$ equals the simulation-based proxy $\mathcal{R}(\theta_0) = \theta_*$. If we denote by $B(\theta; y_{1:n}) = \ell(\theta; y_{1:n}) - \mu(\theta; y_{1:n})$ the Jensen bias at $\theta$ given the observations $y_{1:n}$, we have

$$\mathbb{E}_{Y_{1:n}\sim P^Y_{\theta_0}} \mu(\theta; Y_{1:n}) \le \mathbb{E}_{Y_{1:n}\sim P^Y_{\theta_0}} \ell(\theta; Y_{1:n}) \le \mathbb{E}_{Y_{1:n}\sim P^Y_{\theta_0}} \mu(\theta; Y_{1:n}) + B(\theta; Y_{1:n}),$$

or

$$U(\theta_0, \theta) \le -H(\theta_0, \theta) \le U(\theta_0, \theta) + \mathbb{E}_{Y_{1:n}\sim P^Y_{\theta_0}} B(\theta; Y_{1:n}). \tag{S13}$$

We consider a second order Taylor approximation to $-H(\theta_0, \theta)$ around $\theta = \theta_0$ and an approximation to $U(\theta_0, \theta)$ around $\theta = \theta_*$:

$$\begin{aligned} q_{-H}(\theta) &:= -H(\theta_0, \theta_0) - \frac{1}{2}(\theta - \theta_0)^\top \left[\frac{\partial^2}{\partial\theta^2} H(\theta_0, \theta)\right]_{\theta=\theta_0} (\theta - \theta_0), \\ q_U(\theta) &:= U(\theta_0, \theta_*) + \frac{1}{2}(\theta - \theta_*)^\top \left[\frac{\partial^2}{\partial\theta^2} U(\theta_0, \theta)\right]_{\theta=\theta_*} (\theta - \theta_*). \end{aligned}$$

The first order derivatives of $-H(\theta_0, \theta)$ and $U(\theta_0, \theta)$ evaluated at $\theta_0$ and $\theta_*$, respectively, are equal to zero because those points are the maximizers of the two functions. Note that the second derivative of $H$ at $\theta_0$ equals the Fisher information $\mathcal{I}(\theta_0)$,

$$\left[\frac{\partial^2}{\partial\theta^2} H(\theta_0, \theta)\right]_{\theta=\theta_0} = -\int \left[\frac{\partial^2}{\partial\theta^2} \log p^Y_{\theta,n}(y_{1:n})\right]_{\theta=\theta_0} p^Y_{\theta_0}(y_{1:n})\, \mathrm{d}y_{1:n} = \mathcal{I}(\theta_0).$$

We restate our results from Section 2.5.

Proposition 2. *Suppose that the quadratic approximations $q_{-H}(\theta)$ and $q_U(\theta)$ given by* (12)–(13) *are $\epsilon$-accurate on a $\delta$-neighborhood of $\theta_*$, that is,*

$$|-H(\theta_0, \theta) - q_{-H}(\theta)| \le \epsilon, \quad |U(\theta_0, \theta) - q_U(\theta)| \le \epsilon,$$

*for every $\theta$ such that $\|\theta - \theta_*\| \le \delta$. Suppose further that both the Fisher information $\mathcal{I}(\theta_0)$ and $\mathcal{J}(\theta_0, \theta_*)$ are positive definite and that*

$$\bar{B} := \sup_{\theta; \|\theta-\theta_*\|\le\delta} \mathbb{E}_{Y_{1:n}\sim P^Y_{\theta_0}} B(\theta; Y_{1:n})$$

*is finite. If the smallest eigenvalue $\lambda$ of $\mathcal{J}(\theta_0, \theta_*)$ satisfies $\lambda\delta^2 \ge 2(\bar{B} + 2\epsilon)$, then we have*

$$\|\theta_0 - \theta_*\| \le 2\delta^{-1}\lambda^{-1}(\bar{B} + 2\epsilon).$$

In fact, a somewhat stronger result can be established as follows: the true parameter $\theta_0$ is located in the set

$$\theta_0 \in \{\theta_* + tu;\ u \in \mathbb{R}^d,\ \|u\| = 1,\ |t| \le 2(u^\top \mathcal{J}(\theta_0, \theta_*)u)^{-1}\delta^{-1}(\bar{B} + 2\epsilon)\}. \tag{S14}$$

We note that (S14) implies our original result, $\|\theta_0 - \theta_*\| \le 2\delta^{-1}\lambda^{-1}(\bar{B} + 2\epsilon)$, since $\lambda\|\theta_0 - \theta_*\|^2 \le (\theta_0 - \theta_*)^\top J(\theta_0, \theta_*)(\theta_0 - \theta_*)$. Additionally, we can obtain bounds for the Fisher information as

$$\mathcal{J}(\theta_0, \theta_*) - 2\delta^{-2}(\bar{B} + 2\epsilon)I_d \preceq \mathcal{I}(\theta_0) \preceq \mathcal{J}(\theta_0, \theta_*) + 2\delta^{-2}(\bar{B} + 2\epsilon)I_d,$$

where $A \preceq B$ indicates that $B - A$ is nonnegative definite and $I_d$ denotes the $d \times d$ identity matrix. The proofs of Proposition 2 and these additional results are presented later in this section.

For large $n$, $\mathcal{J}(\theta_0, \theta_*)$ is approximately equal to the metamodel parameter $c$, because

$$-\frac{1}{2}\mathcal{J}(\theta_0, \theta_*) = \frac{1}{2}\left[\frac{\partial^2}{\partial\theta^2} \mathbb{E}_{Y_{1:n}\sim P^Y_{\theta_0}} \mu(\theta; Y_{1:n})\right]_{\theta=\theta_*} \approx \frac{1}{2}\frac{\partial^2}{\partial\theta^2} \mu(\theta_*; y_{1:n}) = c(y_{1:n}).$$

Thus, $\mathcal{J}(\theta_0, \theta_*)$ can be approximately estimated by quadratic regression through the simulated log-likelihoods.

Proposition 3 provides a similar result for the MESLE. For given observation sequence $y_{1:n}$, consider second order Taylor approximations to $\ell(\theta; y_{1:n})$ and $\mu(\theta; y_{1:n})$:

$$q_\ell(\theta) := \ell(\theta_{MLE}) + \frac{1}{2}(\theta - \theta_{MLE})^\top \frac{\partial^2 \ell}{\partial \theta^2}(\theta_{MLE})(\theta - \theta_{MLE}),$$
$$q_\mu(\theta) := \mu(\theta_{MESLE}) + \frac{1}{2}(\theta - \theta_{MESLE})^\top \frac{\partial^2 \mu}{\partial \theta^2}(\theta_{MESLE})(\theta - \theta_{MESLE}).$$

Proposition 3. *Suppose that for a given observation sequence $y_{1:n}$, the quadratic approximations $q_\ell(\theta)$ and $q_\mu(\theta)$ are $\epsilon$-accurate,*

$$|\ell(\theta) - q_\ell(\theta)| \leq \epsilon, \quad |\mu(\theta) - q_\mu(\theta)| \leq \epsilon,$$

*for every $\theta$ such that $\|\theta - \theta_{MESLE}\| \leq \delta$ for some $\epsilon, \delta > 0$. Suppose further that both $-\frac{\partial^2 \ell}{\partial \theta^2}(\theta_{MLE})$ and $-\frac{\partial^2 \mu}{\partial \theta^2}(\theta_{MESLE})$ are positive definite. Let*

$$\bar{B}' := \sup_{\theta; \|\theta - \theta_{MESLE}\| \leq \delta} B(\theta; y_{1:n})$$

*and assume that $\bar{B}'$ is finite. If the smallest eigenvalue $\lambda'$ of $-\frac{\partial^2 \mu}{\partial \theta^2}(\theta_{MESLE})$ satisfies $\lambda' \delta^2 \geq 2(\bar{B}' + 2\epsilon)$, then we have*

$$\|\theta_{MLE} - \theta_{MESLE}\| \leq 2\delta^{-1} {\lambda'}^{-1} (\bar{B}' + 2\epsilon).$$

The conclusion of Proposition 3 is implied by a stronger result

$$\theta_{MLE} \in \left\{ \theta_{MESLE} + tu;\ u \in \mathbb{R}^d,\ \|u\| = 1,\ |t| \leq -2 \left( u^\top \frac{\partial^2 \mu}{\partial \theta^2}(\theta_{MESLE}) u \right)^{-1} \delta^{-1} (\bar{B}' + 2\epsilon) \right\}.$$

Moreover, we have

$$\frac{\partial^2 \mu}{\partial \theta^2}(\theta_{MESLE}) - 2\delta^{-2}(\bar{B}' + 2\epsilon) I_d \preceq \frac{\partial^2 \ell}{\partial \theta^2}(\theta_{MLE}) \preceq \frac{\partial^2 \mu}{\partial \theta^2}(\theta_{MESLE}) + 2\delta^{-2}(\bar{B}' + 2\epsilon) I_d.$$

*Proof of Proposition 2.* From Equation (S13), we have

$$U(\theta_0, \theta) \leq -H(\theta_0, \theta) \leq U(\theta_0, \theta) + \bar{B}$$

for $\theta$ satisfying $\|\theta - \theta_*\| \leq \delta$. Thus we have

$$\begin{aligned} q_{-H}(\theta) &\geq -H(\theta_0, \theta) - \epsilon \geq U(\theta_0, \theta) - \epsilon \geq q_U(\theta) - 2\epsilon, \\ q_{-H}(\theta) &\leq -H(\theta_0, \theta) + \epsilon \leq U(\theta_0, \theta) + \bar{B} + \epsilon \leq q_U(\theta) + \bar{B} + 2\epsilon. \end{aligned} \tag{S15}$$

Let

$$v = \frac{\theta_0 - \theta_*}{\|\theta_0 - \theta_*\|}$$

be a unit vector in the direction from $\theta_*$ to $\theta_0$. Define $r_U : [-\delta, \delta] \to \mathbb{R}$ and $r_{-H} : [-\delta, \delta] \to \mathbb{R}$ by

$$r_U(x) = q_U(\theta_* + xv) - q_U(\theta_*) = -\nu x^2$$

and

$$r_{-H}(x) = q_{-H}(\theta_* + xv) - q_U(\theta_*) = -\alpha(x - \beta)^2 + \gamma.$$

Here,

$$2\nu = -\frac{d^2}{dx^2} r_U(x) = -v^\top \frac{\partial^2}{\partial \theta^2} q_U(\theta) v = v^\top \mathcal{J}(\theta_0, \theta_*) v \geq \lambda,$$

$$2\alpha = -\frac{d}{dx^2} r_{-H}(x) = -v^\top \frac{\partial^2}{\partial \theta^2} q_{-H}(\theta) v = v^\top \mathcal{I}(\theta_0) v.$$

Also, $\beta = \|\theta_0 - \theta_*\|$, because $r_{-H}(x)$ is maximized at $x = \beta$ and $q_{-H}(\theta)$ is maximized at $\theta = \theta_0$ by construction. From (S15), we have envelopes for $r_{-H}(x)$:

$$r_U(x) - 2\epsilon \le r_{-H}(x) \le r_U(x) + \bar{B} + 2\epsilon \tag{S16}$$

for $|x| \le \delta$. Additionally, we have

$$0 \le -H(\theta_0, \theta_*) - U(\theta_0, \theta_*) \le \gamma = -H(\theta_0) - U(\theta_0, \theta_*) \le -H(\theta_0) - U(\theta_0, \theta_0) \le \bar{B}.$$

We consider two separate cases. In the case $\alpha \le \nu$, Equation (S16) implies that

$$r_{-H}(\delta) = -\alpha(x - \beta)^2 + \gamma \le r_U(\delta) + \bar{B} + 2\epsilon = -\nu\delta^2 + \bar{B} + 2\epsilon.$$

Thus we have

$$(\delta - \beta)^2 \ge \alpha^{-1}(\nu\delta^2 - \bar{B} - 2\epsilon + \gamma), \tag{S17}$$

or

$$\beta \le \delta - \sqrt{\alpha^{-1}(\nu\delta^2 - \bar{B} - 2\epsilon + \gamma)}$$
$$\le \delta - \sqrt{\delta^2 - \nu^{-1}(\bar{B} + 2\epsilon - \gamma)} = \delta - \delta\sqrt{1 - \delta^{-2}\nu^{-1}(\bar{B} + 2\epsilon - \gamma)}.$$

Since $\nu\delta^2 \ge \frac{\lambda}{2}\delta^2 \ge \bar{B} + 2\epsilon \ge \bar{B} + 2\epsilon - \gamma$, the expression inside the square root symbol is nonnegative. Using the fact that $\sqrt{1-t} \ge 1 - t$ for $0 \le t \le 1$, we obtain

$$\beta \le \delta - \delta\{1 - \delta^{-2}\nu^{-1}(\bar{B} + 2\epsilon - \gamma)\} \le \delta^{-1}\nu^{-1}(\bar{B} + 2\epsilon).$$

Now consider the case $\alpha > \nu$. Equation (S16) implies that

$$r_{-H}(-\delta) = -\alpha(-\delta - \beta)^2 + \gamma \ge r_U(-\delta) - 2\epsilon = -nu(-\delta)^2 - 2\epsilon.$$

Thus we have

$$(\delta + \beta)^2 \le \alpha^{-1}(\nu\delta^2 + \gamma + 2\epsilon), \tag{S18}$$

or

$$\beta \le \sqrt{\alpha^{-1}(\nu\delta^2 + \gamma + 2\epsilon)} - \delta \le \sqrt{\delta^2 + \nu^{-1}(\gamma + 2\epsilon)} - \delta = \delta\sqrt{1 + \delta^{-2}\nu^{-1}(\gamma + 2\epsilon)} - \delta.$$

Using the fact that $\sqrt{1+t} \le 1 + \frac{t}{2}$ for $t \ge 0$, we obtain

$$\beta \le \delta\{1 + \frac{1}{2}\delta^{-2}\nu^{-1}(\gamma + 2\epsilon)\} - \delta \le \delta^{-1}\nu^{-1}(\bar{B} + 2\epsilon).$$

In either case, we have

$$\beta = \|\theta_0 - \theta_*\| \le \delta^{-1}\nu^{-1}(\bar{B} + 2\epsilon) = 2(v^\top \mathcal{J}(\theta_0, \theta_*)v)^{-1}\delta^{-1}(\bar{B} + 2\epsilon).$$

In other words, $\theta_0$ is located in the set

$$\theta_0 \in \{\theta_* + tu;\ u \in \mathbb{R}^d,\ \|u\| = 1,\ |t| \le 2(u^\top \mathcal{J}(\theta_0, \theta_*)u)^{-1}\delta^{-1}(\bar{B} + 2\epsilon)\}.$$

We now prove the bounds on the Fisher information $\mathcal{I}(\theta_0)$. Using (S17) again, we have

$$\alpha \ge (\delta - \beta)^{-2}(\nu\delta^2 - \bar{B} - 2\epsilon + \gamma) \ge \nu - \delta^{-2}(\bar{B} + 2\epsilon - \gamma) \ge \nu - \delta^{-2}(\bar{B} + 2\epsilon).$$

This implies that

$$\frac{1}{2}v^\top \mathcal{I}(\theta_0)v \ge \frac{1}{2}v^\top \mathcal{J}(\theta_0, \theta_*)v - \delta^{-2}(\bar{B} + 2\epsilon).$$

From (S18), we have

$$\alpha \le (\delta + \beta)^{-2}(\nu\delta^2 + \gamma + 2\epsilon) \le \nu + \delta^{-2}(\gamma + 2\epsilon) \le \nu + \delta^{-2}(\bar{B} + 2\epsilon),$$

which implies that

$$\frac{1}{2}v^\top \mathcal{I}(\theta_0)v \le \frac{1}{2}v^\top \mathcal{J}(\theta_0,\theta_*)v + \delta^{-2}(\bar{B}+2\epsilon).$$

We can obtain the same results when we replace $v$ by an arbitrary unit vector $u$. Hence, we have

$$\mathcal{J}(\theta_0,\theta_*) - 2\delta^{-2}(\bar{B}+2\epsilon)I_d \preceq \mathcal{I}(\theta_0) \preceq \mathcal{J}(\theta_0,\theta_*) - 2\delta^{-2}(\bar{B}+2\epsilon)I_d.$$

□

The proof of Proposition 3 follows similarly and is thus omitted.

# S4 Mathematical details and proofs for Section 3

## S4.1 Details and proofs for Section 3.1

The $MLLR_{A_0,\sigma_0^2}$ statistic for the test $H_0 : A = A_0, \sigma^2 = \sigma_0^2$, $H_1$ : not $H_0$ has the following distribution under the null hypothesis.

**Proposition S4.** *Under the normal, locally quadratic metamodel (Definition 3) and under the null hypothesis $A = A_0$ and $\sigma^2 = \sigma_0^2$, the metamodel log-likelihood ratio* (16) *has the following distribution:*

$$MLLR_{A_0,\sigma_0^2} \sim \mathsf{SCL}\left(M, \frac{d^2+3d+2}{2}\right).$$

**Definition S2** ($\mathsf{SCL}$ distributions)**.** Let $X_1 \sim \chi^2_k$ and $X_2 \sim \chi^2_{M-k}$ be independent random variables following the chi-squared distributions with $k$ and $M-k$ degrees of freedom. Then the distribution of the random variable

$$-\frac{1}{2}\left\{X_1 + X_2 - M\log\frac{X_2}{M} - M\right\} \tag{S19}$$

will called the $\mathsf{SCL}(M,k)$ distribution.[1]

The $-2\cdot\mathsf{SCL}(M,k)$ distribution converges to the chi-square distribution as $M$ tends to infinity.

**Proposition S5.** *As $M$ tends to infinity, we have*

$$-2\cdot\mathsf{SCL}(M,k) \underset{M\to\infty}{\Longrightarrow} \chi^2_{k+1}.$$

Propositions S4 and S5 show that our metamodel likelihood ratio test is asymptotically equivalent to Wilks' large-sample likelihood ratio test as the number of simulations $M$ grows.

**Lemma S2.** *The sum of squared errors can be divided into the residual sum of squares and the squared error in fit as follows:*

$$\|\ell^S_{1:M} - \theta^{0:2}_{1:M}A_0\|^2_W = \|\ell^S_{1:M} - \theta^{0:2}_{1:M}\hat{A}\|^2_W + \|\theta^{0:2}_{1:M}\hat{A} - \theta^{0:2}_{1:M}A_0\|^2_W. \tag{S20}$$

*Furthermore, under the null hypothesis $A = A_0$ and $\sigma^2 = \sigma_0^2$ for the normal, locally quadratic metamodel, we have*

$$\hat{\sigma}^2 \sim \frac{1}{M}\sigma_0^2\chi^2_{M-\frac{d^2+3d+2}{2}} \qquad \text{and} \qquad \|\theta^{0:2}_{1:M}\hat{A} - \theta^{0:2}_{1:M}A_0\|^2_W \sim \sigma_0^2\chi^2_{\frac{d^2+3d+2}{2}},$$

*and these two random variables are independent, provided that $\theta^{0:2}_{1:M}$ has rank $\frac{d^2+3d+2}{2}$.*

*Proof of Lemma S2.* The decomposition of the sum of squared errors given by (S20) is a common result in regression analysis, see e.g., Agresti [2, Section 2.2.5]. Define a random vector $\mathbf{Z} = (Z_1,\ldots,Z_M)$ such that

$$\ell^S_{1:M} = \theta^{0:2}_{1:M}A_0 + \sigma_0 W^{-1/2}\mathbf{Z}.$$

[1] This distribution is named $\mathsf{SCL}$ because it is the distribution of the Sum of a Chi-squared random variate and the Log of another chi-squared random variate.

For our normal, locally quadratic metamodel (Definition 3) under $H_0 : A = A_0,\ \sigma^2 = \sigma_0^2$, the $M$ components of $\mathbf{Z}$ are standard normal random variates and are independent of each other. We have

$$\begin{aligned}\hat{A} &= ({\theta_{1:M}^{0:2}}^\top W \theta_{1:M}^{0:2})^{-1} {\theta_{1:M}^{0:2}}^\top W \ell_{1:M}^S \\ &= ({\theta_{1:M}^{0:2}}^\top W \theta_{1:M}^{0:2})^{-1} {\theta_{1:M}^{0:2}}^\top W (\theta_{1:M}^{0:2} A_0 + \sigma_0 W^{-1/2}\mathbf{Z}) \\ &= A_0 + \sigma_0 ({\theta_{1:M}^{0:2}}^\top W \theta_{1:M}^{0:2})^{-1} {\theta_{1:M}^{0:2}}^\top W^{1/2}\mathbf{Z}.\end{aligned} \tag{S21}$$

Thus

$$\begin{aligned}&\ell_{1:M}^S - \theta_{1:M}^{0:2}\hat{A} \\ &= \theta_{1:M}^{0:2} A_0 + \sigma_0 W^{-1/2}\mathbf{Z} - \theta_{1:M}^{0:2} A_0 - \sigma_0 \theta_{1:M}^{0:2} ({\theta_{1:M}^{0:2}}^\top W \theta_{1:M}^{0:2})^{-1} {\theta_{1:M}^{0:2}}^\top W^{1/2}\mathbf{Z} \\ &= \sigma_0 W^{-1/2}(I - W^{1/2}\theta_{1:M}^{0:2} ({\theta_{1:M}^{0:2}}^\top W \theta_{1:M}^{0:2})^{-1} {\theta_{1:M}^{0:2}}^\top W^{1/2})\mathbf{Z}.\end{aligned}$$

Let $H_w := W^{1/2}\theta_{1:M}^{0:2} ({\theta_{1:M}^{0:2}}^\top W \theta_{1:M}^{0:2})^{-1} {\theta_{1:M}^{0:2}}^\top W^{1/2}$. This matrix is an orthogonal projection matrix, that is, $H_w^\top = H_w$ and $H_w^2 = H_w$. It can be readily checked that $I - H_w$ is also an orthogonal projection matrix. The rank of $H_w$ is $\frac{d^2+3d+2}{2}$ because we assume that $\theta_{1:M}^{0:2}$ has rank $\frac{d^2+3d+2}{2}$. The distribution of $\hat{\sigma}^2$ can be expressed as

$$\hat{\sigma}^2 = \frac{1}{M}\|\ell_{1:M}^S - \theta_{1:M}^{0:2}\hat{A}\|_W^2 = \frac{1}{M}\sigma_0^2 \mathbf{Z}^\top (I - H_w)\mathbf{Z} \sim \frac{1}{M}\sigma_0^2 \chi^2_{M - \frac{d^2+3d+2}{2}},$$

because $I - H_w$ can be orthogonally diagonalizable with $M - \frac{d^2+3d+2}{2}$ eigenvalues equal to 1 and $\frac{d^2+3d+2}{2}$ eigenvalues equal to 0. One can also check that

$$\|\theta_{1:M}^{0:2}\hat{A} - \theta_{1:M}^{0:2}A_0\|_W^2 \overset{d}{=} \sigma_0^2 \mathbf{Z}^\top H_w \mathbf{Z} \sim \sigma_0^2 \chi^2_{\frac{d^2+3d+2}{2}}.$$

Two random variables $H_w\mathbf{Z}$ and $(I - H_w)\mathbf{Z}$ are uncorrelated, because $H_w(I - H_w) = 0$. Thus $\hat{\sigma}^2 = \frac{\sigma_0^2}{M}\mathbf{Z}^\top (I - H_w)(I - H_w)\mathbf{Z}$ and $\|\theta_{1:M}^{0:2}\hat{A} - \theta_{1:M}^{0:2}A_0\|_W^2 = \sigma_0^2 \mathbf{Z}^\top H_w H_w \mathbf{Z}$ are independent. □

*Proof of Proposition S4.* Let

$$X_1 = \frac{\|\theta_{1:M}^{0:2}\hat{A} - \theta_{1:M}^{0:2}A_0\|_W^2}{\sigma_0^2}, \quad X_2 = \frac{\|\ell_{1:M}^S - \theta_{1:M}^{0:2}\hat{A}\|_W^2}{\sigma_0^2} = \frac{M\hat{\sigma}^2}{\sigma_0^2}.$$

By Lemma S2, we see that $X_1 \sim \chi^2_{\frac{d^2+3d+2}{2}}$, $X_2 \sim \chi^2_{M-\frac{d^2+3d+2}{2}}$ are independent and that $X_1 + X_2 = \|\ell_{1:M}^S - \theta_{1:M}^{0:2}\hat{A}\|_W^2$. The metamodel log likelihood ratio statistic can be expressed as

$$\begin{aligned}MLLR_{A_0,\sigma_0^2} &= \frac{M}{2}\log\frac{\hat{\sigma}^2}{\sigma_0^2} - \frac{\|\hat{\ell}_{1:M}^{SB} - \theta_{1:M}^{0:2}A_0\|_W^2}{2\sigma_0^2} + \frac{M}{2} \\ &= -\frac{X_1 + X_2}{2} + \frac{M}{2}\log\frac{X_2}{M} + \frac{M}{2} \\ &\sim \mathsf{SCL}(M, \frac{d^2+3d+2}{2}).\end{aligned}$$

□

*Proof of Proposition S5.* Since $X_2 \sim \chi^2_{M-k}$ has the same distribution as that of the sum of $M-k$ independent squares of standard normal random variates, it can be readily seen by the central limit theorem that

$$\sqrt{M}\left(\frac{X_2}{M} - 1\right) \underset{M\to\infty}{\Longrightarrow} \mathcal{N}(0, 2).$$

Using the Taylor expansion $\log(1+\epsilon) = \epsilon - \frac{\epsilon^2}{2} + O(\epsilon^3)$, we see that

$$\log\frac{X_2}{M} = \frac{X_2}{M} - 1 - \frac{1}{2}\left(\frac{X_2}{M} - 1\right)^2 + O_p\left(\frac{1}{\sqrt{M}^3}\right).$$

Therefore,

$$\begin{aligned} X_2 - M - M\log\frac{X_2}{M} &= X_2 - M - M\left[\frac{X_2}{M} - 1 - \frac{1}{2}\left(\frac{X_2}{M}-1\right)^2 + O_p\left(\frac{1}{\sqrt{M}^3}\right)\right] \\ &= \frac{M}{2}\left(\frac{X_2}{M}-1\right)^2 + O_p\left(\frac{1}{\sqrt{M}}\right) \\ &\underset{M\to\infty}{\Longrightarrow} \chi_1^2. \end{aligned}$$

Thus if $X_1 \sim \chi_k^2$ is independent of $X_2$,

$$-2\cdot \mathsf{SCL}(M,k) \overset{d}{=} X_1 + X_2 - M\log\frac{X_2}{M} - M \Longrightarrow \chi_{k+1}^2.$$

□

## S4.2 Details and proofs for Section 3.2

*Proof of Proposition 4.* For an arbitrary vector $\mathbf{v} = (\mathbf{v}_1^\top, \mathbf{v}_2^\top)^\top \in \mathbb{R}^{n_1+n_2}$ with $\mathbf{v}_1 \in \mathbb{R}^{n_1}$ and $\mathbf{v}_2 \in \mathbb{R}^{n_2}$ and a symmetric positive definite matrix $B = \begin{pmatrix} B_{11} & B_{12} \\ B_{12}^\top & B_{22}\end{pmatrix}$ with $B_{11} \in \mathbb{R}^{n_1\times n_1}$ and $B_{22} \in \mathbb{R}^{n_2\times n_2}$, the following holds:

$$\min_{\mathbf{v}_1} \mathbf{v}^\top B\mathbf{v} = \min_{\mathbf{v}_1} \begin{pmatrix}\mathbf{v}_1\\ \mathbf{v}_2\end{pmatrix}^\top \begin{pmatrix} B_{11} & B_{12} \\ B_{12}^\top & B_{22}\end{pmatrix}\begin{pmatrix}\mathbf{v}_1\\ \mathbf{v}_2\end{pmatrix} = \mathbf{v}_2^\top\left(B_{22} - B_{12}^\top B_{11}^{-1}B_{12}\right)\mathbf{v}_2.$$

From the fact that

$$U = \begin{pmatrix} u_{aa} & \mathbf{u}_{a,bc} \\ \mathbf{u}_{bc,a} & U_{bc,bc}\end{pmatrix} := {\theta_{1:M}^{0:2}}^\top W\theta_{1:M}^{0:2} = \left(\textstyle\sum_{m=1}^M w_m\right)\cdot\begin{pmatrix} 1 & \overline{\theta} & \overline{\theta^2} \\ \overline{\theta} & \overline{\theta^2} & \overline{\theta^3} \\ \overline{\theta^2} & \overline{\theta^3} & \overline{\theta^4}\end{pmatrix},$$

it follows that

$$\begin{aligned} \min_{a_0} \|\theta_{1:M}^{0:2}\hat{A} - \theta_{1:M}^{0:2}A_0\|_W^2 &= \min_{a_0} (\hat{A}-A_0)^\top U(\hat{A}-A_0) \\ &= \begin{pmatrix}\hat{b}-b_0 \\ \mathrm{vech}(\hat{c}) - \mathrm{vech}(c_0)\end{pmatrix} V \begin{pmatrix}\hat{b}-b_0 \\ \mathrm{vech}(\hat{c}) - \mathrm{vech}(c_0)\end{pmatrix} \end{aligned} \tag{S22}$$

where

$$V := U_{bc,bc} - \mathbf{u}_{bc,a}u_{aa}^{-1}\mathbf{u}_{a,bc}.$$

We can find

$$\min_{-\frac{1}{2}c_0^{-1}b_0 = \theta_{H_0}} \begin{pmatrix}\hat{b}-b_0 \\ \mathrm{vech}(\hat{c}) - \mathrm{vech}(c_0)\end{pmatrix} V \begin{pmatrix}\hat{b}-b_0 \\ \mathrm{vech}(\hat{c}) - \mathrm{vech}(c_0)\end{pmatrix}$$

using the method of Lagrange multiplier. Let

$$\mathcal{L} = \begin{pmatrix}\hat{b}-b_0 \\ \mathrm{vech}(\hat{c}) - \mathrm{vech}(c_0)\end{pmatrix}^\top V \begin{pmatrix}\hat{b}-b_0 \\ \mathrm{vech}(\hat{c}) - \mathrm{vech}(c_0)\end{pmatrix} + \lambda^\top(2\theta_{H_0,\mathrm{mat}}\mathrm{vech}(c_0) + b_0)$$

for $\lambda \in \mathbb{R}^d$. We find

$$\begin{aligned} \left(\frac{\partial\mathcal{L}}{\partial b_0}\right)^\top &= 2V_{bb}(b_0 - \hat{b}) - 2V_{bc}(\mathrm{vech}(\hat{c}) - \mathrm{vech}(c_0)) + \lambda, \\ \left(\frac{\partial\mathcal{L}}{\partial \mathrm{vech}(c_0)}\right)^\top &= -2V_{cb}(\hat{b} - b_0) - 2V_{cc}(\mathrm{vech}(\hat{c}) - \mathrm{vech}(c_0)) + 2\theta_{H_0,\mathrm{mat}}^\top\lambda. \end{aligned}$$

Equating both expression to zero gives

$$V_{cb}(b_0 - \hat{b}) + V_{cc}(\mathrm{vech}(c_0) - \mathrm{vech}(\hat{c})) = \theta_{H_0,\mathrm{mat}}^\top \{2V_{bb}(b_0 - \hat{b}) + 2V_{bc}(\mathrm{vech}(c_0) - \mathrm{vech}(\hat{c}))\}.$$

Thus by writing

$$V_1 := V_{cb} - 2\theta_{H_0,\mathrm{mat}}^\top V_{bb}, \qquad V_2 := V_{cc} - 2\theta_{H_0,\mathrm{mat}}^\top V_{bc},$$

we have

$$V_1(b_0 - \hat{b}) + V_2(\mathrm{vech}(c_0) - \mathrm{vech}(\hat{c})) = 0.$$

By using the constraint $2\theta_{H_0,\mathrm{mat}}\mathrm{vech}(c_0) + b_0 = 0$, we obtain

$$\begin{aligned}\mathrm{vech}(c_0) &= (V_2 - 2V_1\theta_{H_0,\mathrm{mat}})^{-1}(V_1\hat{b} + V_2\mathrm{vech}(\hat{c})),\\ b_0 &= -2\theta_{H_0,\mathrm{mat}}(V_2 - 2V_1\theta_{H_0,\mathrm{mat}})^{-1}(V_1\hat{b} + V_2\mathrm{vech}(\hat{c})).\end{aligned}$$

We will write

$$\begin{aligned}V_- := V_2 - 2V_1\theta_{H_0,\mathrm{mat}} &= V_{cc} - 2\theta_{H_0,\mathrm{mat}}^\top V_{bc} - 2V_{cb}\theta_{H_0,\mathrm{mat}} + 4\theta_{H_0,\mathrm{mat}}^\top V_{bb}\theta_{H_0,\mathrm{mat}}\\ &= \begin{pmatrix}-2\theta_{H_0,\mathrm{mat}}^\top & I_{\frac{d^2+d}{2}}\end{pmatrix}\begin{pmatrix}V_{bb} & V_{bc}\\ V_{cb} & V_{cc}\end{pmatrix}\begin{pmatrix}-2\theta_{H_0,\mathrm{mat}}\\ I_{\frac{d^2+d}{2}}\end{pmatrix},\end{aligned}$$

We then have

$$\begin{aligned}\begin{pmatrix}b_0\\ \mathrm{vech}(c_0)\end{pmatrix} &= \begin{pmatrix}-2\theta_{H_0,\mathrm{mat}}V_-^{-1}V_1 & -2\theta_{H_0,\mathrm{mat}}V_-^{-1}V_2\\ V_-^{-1}V_1 & V_-^{-1}V_2\end{pmatrix}\begin{pmatrix}\hat{b}\\ \mathrm{vech}(\hat{c})\end{pmatrix}\\ &= \begin{pmatrix}-2\theta_{H_0,\mathrm{mat}}\\ I_{\frac{d^2+d}{2}}\end{pmatrix} V_-^{-1}\begin{pmatrix}-2\theta_{H_0,\mathrm{mat}}^\top & I_{\frac{d^2+d}{2}}\end{pmatrix} V \begin{pmatrix}\hat{b}\\ \mathrm{vech}(\hat{c})\end{pmatrix}.\end{aligned}$$

By plugging in this solution to the constrained optimization problem, we find

$$\begin{aligned}&\min_{-\frac{1}{2}c_0^{-1}b_0=\theta_{H_0}}\begin{pmatrix}\hat{b} - b_0\\ \mathrm{vech}(\hat{c}) - \mathrm{vech}(c_0)\end{pmatrix}^\top V\begin{pmatrix}\hat{b} - b_0\\ \mathrm{vech}(\hat{c}) - \mathrm{vech}(c_0)\end{pmatrix}\\ &= \left\{I_{\frac{d^2+3d}{2}} - \begin{pmatrix}-2\theta_{H_0,\mathrm{mat}}\\ I_{\frac{d^2+d}{2}}\end{pmatrix}V_-^{-1}\begin{pmatrix}-2\theta_{H_0,\mathrm{mat}}^\top & I_{\frac{d^2+d}{2}}\end{pmatrix}V\begin{pmatrix}\hat{b}\\ \mathrm{vech}(\hat{c})\end{pmatrix}\right\}^\top V\\ &\quad \left\{I_{\frac{d^2+3d}{2}} - \begin{pmatrix}-2\theta_{H_0,\mathrm{mat}}\\ I_{\frac{d^2+d}{2}}\end{pmatrix}V_-^{-1}\begin{pmatrix}-2\theta_{H_0,\mathrm{mat}}^\top & I_{\frac{d^2+d}{2}}\end{pmatrix}V\begin{pmatrix}\hat{b}\\ \mathrm{vech}(\hat{c})\end{pmatrix}\right\}\\ &= V - V\begin{pmatrix}-2\theta_{H_0,\mathrm{mat}}\\ I_{\frac{d^2+d}{2}}\end{pmatrix}V_-^{-1}\begin{pmatrix}-2\theta_{H_0,\mathrm{mat}}^\top & I_{\frac{d^2+d}{2}}\end{pmatrix}V.\end{aligned}$$

Using Lemma S3, we can express this constrained minimum as

$$\begin{pmatrix}I_d\\ 2\theta_{H_0,\mathrm{mat}}^\top\end{pmatrix}\left\{\begin{pmatrix}I & 2\theta_{H_0,\mathrm{mat}}\end{pmatrix}V^{-1}\begin{pmatrix}I\\ 2\theta_{H_0,\mathrm{mat}}^\top\end{pmatrix}\right\}^{-1}\begin{pmatrix}I_d & 2\theta_{H_0,\mathrm{mat}}\end{pmatrix}, \tag{S23}$$

The $MLLR_{\theta_{H_0}}$ statistic is given by

$$\begin{aligned}MLLR_{\theta_{H_0}} &= \sup_{\sigma_0^2>0}\sup_{-\frac{1}{2}c_0^{-1}b_0=\theta_{H_0}}\frac{M}{2}\log\frac{\hat{\sigma}^2}{\sigma_0^2} - \frac{M\hat{\sigma}^2}{2\sigma_0^2} - \frac{\|\theta_{1:M}^{0:2}\hat{A} - \theta_{1:M}^{0:2}A_0\|_W^2}{2\sigma_0^2} + \frac{M}{2}\\ &= \sup_{\sigma_0^2>0}\frac{M}{2}\log\frac{\hat{\sigma}^2}{\sigma_0^2} - \frac{M\hat{\sigma}^2}{2\sigma_0^2} - \frac{\xi}{2\sigma_0^2} + \frac{M}{2}\\ &= \frac{M}{2}\log\frac{\hat{\sigma}^2}{\hat{\sigma}^2 + M^{-1}\xi} = -\frac{M}{2}\log\left(\frac{\xi}{M\hat{\sigma}^2} + 1\right).\end{aligned}$$

In the proof of Lemma S2, we showed that

$$\hat{A} = A_0 + \sigma_0({\theta^{0:2}_{1:M}}^\top W \theta^{0:2}_{1:M})^{-1}{\theta^{0:2}_{1:M}}^\top W^{1/2}\mathbf{Z}$$

where $\mathbf{Z} \sim \mathcal{N}(0, I_M)$. Thus we have

$$\begin{aligned}\hat{b} + 2\hat{c}\theta_{H_0} &= (\mathbf{0}_d,\, I_d,\, 2\theta_{H_0,\mathrm{mat}})\hat{A}\\ &= \sigma_0 \cdot (\mathbf{0}_d,\, I_d,\, 2\theta_{H_0,\mathrm{mat}})U^{-1}{\theta^{0:2}_{1:M}}^\top W^{1/2}\mathbf{Z},\end{aligned}$$

since we assume $(\mathbf{0}_d,\, I_d,\, 2\theta_{H_0,\mathrm{mat}})A_0 = b_0 + 2c_0\theta_{H_0} = 0$. Hence,

$$\hat{b} + 2\hat{c}\theta_{H_0} \sim \mathcal{N}\{0,\, \sigma_0^2 \cdot (\mathbf{0}_d,\, I_d,\, 2\theta_{H_0,\mathrm{mat}})U^{-1}(\mathbf{0}_d,\, I_d,\, 2\theta_{H_0,\mathrm{mat}})^\top\}$$

Using the block matrix inversion formula [10], we see that when the first row and the first column of $U^{-1}$ are removed, we obtain $V^{-1}$:

$$U^{-1} = \begin{pmatrix} * & * & * \\ * & & \\ * & \multicolumn{2}{c}{V^{-1}} \end{pmatrix}.$$

Thus

$$\hat{b} + 2\hat{c}\theta_{H_0} \sim \mathcal{N}\{0,\, \sigma_0^2 \cdot (I_d,\, 2\theta_{H_0,\mathrm{mat}})V^{-1}(I_d,\, 2\theta_{H_0,\mathrm{mat}})^\top\}$$

Therefore, we have

$$\xi = (\hat{b} + 2\hat{c}\theta_{H_0})^\top \left\{ \begin{pmatrix} I_d \\ 2\theta_{H_0,\mathrm{mat}}^\top \end{pmatrix}^\top V^{-1} \begin{pmatrix} I_d \\ 2\theta_{H_0,\mathrm{mat}}^\top \end{pmatrix} \right\}^{-1} (\hat{b} + 2c_0\theta_{H_0}) \sim \sigma_0^2\chi_d^2.$$

Furthermore, we showed in Lemma S2 that $M\hat{\sigma}^2 \sim \sigma_0^2\chi^2_{M-\frac{d^2+3d+2}{2}}$ and that $\hat{A}$ and $\hat{\sigma}^2$ are independent. It follows that

$$\frac{(M - \frac{d^2+3d+2}{2})\xi}{Md\hat{\sigma}^2} \sim F_{d, M-\frac{d^2+3d+2}{2}}.$$

□

**Lemma S3.** *Let* $V = \begin{pmatrix} V_{11} & V_{12} \\ V_{21} & V_{22} \end{pmatrix}$ *be a block matrix with* $V_{11} \in \mathbb{R}^{d_1 \times d_1}$ *and* $V_{22} \in \mathbb{R}^{d_2 \times d_2}$. *If* $V$ *and* $V_{11}$ *are invertible, then for any matrix* $B \in \mathbb{R}^{d_1 \times d_2}$, *we have*

$$\begin{aligned}&\begin{pmatrix} I_{d_1} \\ B^\top \end{pmatrix} \left\{ \begin{pmatrix} I_{d_1} & B \end{pmatrix} V^{-1} \begin{pmatrix} I_{d_1} \\ B^\top \end{pmatrix} \right\}^{-1} \begin{pmatrix} I_{d_1} & B \end{pmatrix}\\ &\qquad = V - V \begin{pmatrix} -B \\ I_{d_2} \end{pmatrix} \left\{ \begin{pmatrix} -B^\top & I_{d_2} \end{pmatrix} V \begin{pmatrix} -B \\ I_{d_2} \end{pmatrix} \right\}^{-1} \begin{pmatrix} -B^\top & I_{d_2} \end{pmatrix} V. \quad \text{(S24)}\end{aligned}$$

*Proof.* Writing $V_{2|1} := V_{22} - V_{21}V_{11}^{-1}V_{12}$, we have, according to Lu and Shiou [10, Theorem 2.1], that

$$V^{-1} = \begin{pmatrix} V_{11}^{-1} + V_{11}^{-1}V_{12}V_{2|1}^{-1}V_{21}V_{11}^{-1} & -V_{11}^{-1}V_{12}V_{2|1}^{-1} \\ -V_{2|1}^{-1}V_{21}V_{11}^{-1} & V_{2|1}^{-1} \end{pmatrix}.$$

Thus we can write

$$\begin{pmatrix} I_{d_1} & B \end{pmatrix} V^{-1} \begin{pmatrix} I_{d_1} \\ B^\top \end{pmatrix} = V_{11}^{-1} + \begin{pmatrix} I_{d_1} & B \end{pmatrix} \begin{pmatrix} V_{11}^{-1}V_{12} \\ -I_{d_2} \end{pmatrix} V_{2|1}^{-1} \begin{pmatrix} V_{21}V_{11}^{-1} & -I_{d_2} \end{pmatrix} \begin{pmatrix} I_{d_1} \\ B^\top \end{pmatrix}$$

Using the Sherman-Morrison-Woodbury formula [14]

$$(A + BCD)^{-1} = A^{-1} - A^{-1}B(C^{-1} + DA^{-1}B)^{-1}DA^{-1},$$

we have

$$\begin{aligned}
&\left\{V_{11}^{-1} + \begin{pmatrix} I_{d_1} & B \end{pmatrix} \begin{pmatrix} V_{11}^{-1}V_{12} \\ -I_{d_2} \end{pmatrix} V_{2|1}^{-1} \begin{pmatrix} V_{21}V_{11}^{-1} & -I_{d_1} \end{pmatrix} \begin{pmatrix} I_{d_1} \\ B^\top \end{pmatrix} \right\}^{-1} \\
&= V_{11} - V_{11}(V_{11}^{-1}V_{12} - B)\{V_{2|1} + (V_{21}V_{11}^{-1} - B^\top)V_{11}(V_{11}^{-1}V_{12} - B)\}^{-1}(V_{21}V_{11}^{-1} - B^\top)V_{11} \\
&= V_{11} - (V_{12} - V_{11}B)\left\{\begin{pmatrix} -B^\top & I_{d_2} \end{pmatrix} V \begin{pmatrix} -B \\ I_{d_2} \end{pmatrix}\right\}^{-1} (V_{21} - B^\top V_{11}),
\end{aligned}$$

showing that the top-left matrix blocks for the left and the right hand sides of (S24) agree. To show that the bottom-left matrix blocks agree, we need to show that the bottom-left matrix block of the right hand side of (S24) is obtained by multiplying $B^\top$ on the left of the top-left block. This can be checked by observing that

$$\begin{pmatrix} -B^\top & I_{d_2} \end{pmatrix} \left[ V - V \begin{pmatrix} -B \\ I_{d_2} \end{pmatrix} \left\{ \begin{pmatrix} -B^\top & I_{d_2} \end{pmatrix} V \begin{pmatrix} -B \\ I_{d_2} \end{pmatrix} \right\}^{-1} \begin{pmatrix} -B^\top & I_{d_2} \end{pmatrix} V \right] = 0.$$

The fact that the top-right and the bottom-right blocks agree on either side of (S24) can be shown by the fact that

$$\left[ V - V \begin{pmatrix} -B \\ I_{d_2} \end{pmatrix} \left\{ \begin{pmatrix} -B^\top & I_{d_2} \end{pmatrix} V \begin{pmatrix} -B \\ I_{d_2} \end{pmatrix} \right\}^{-1} \begin{pmatrix} -B^\top & I_{d_2} \end{pmatrix} V \right] \begin{pmatrix} -B \\ I_{d_2} \end{pmatrix} = 0.$$

□

*Proof of Corollary 1.* Proposition 4 shows that for $d = 1$, $H_0 : \theta_{MESLE} = \theta_{H_0}$ is not rejected at level $\alpha$ if

$$\xi = \frac{M-3}{M\hat{\sigma}^2} \frac{(\hat{b} + 2\hat{c}\theta_{H_0})^2 (V_{bb}V_{cc} - V_{bc}^2)}{V_{cc} - 4V_{bc}\theta_{H_0} + 4V_{bb}\theta_{H_0}^2} < F_{1,M-3,\alpha}.$$

Rearranging the terms, we see that a level $1 - \alpha$ confidence interval for $\theta_{MESLE}$ is given by

$$\begin{aligned}
\big\{\theta;\ &\big[4(M-3)\hat{c}^2 \det V - 4M\hat{\sigma}^2 F_{1,M-3,\alpha} V_{bb}\big]\theta^2 \\
&\qquad + \big[4(M-3)\hat{b}\hat{c} \det V + 4M\hat{\sigma}^2 F_{1,M-3,\alpha} V_{bc}\big]\theta \\
&\qquad\qquad + (M-3)\hat{b}^2 \det V - M\hat{\sigma}^2 F_{1,M-3,\alpha} V_{cc} < 0\big\},
\end{aligned}$$

where $\det V = V_{bb}V_{cc} - V_{bc}^2$. □

# S5 Mathematical details and proofs for Section 4

We have from Section 4 that

$$C\ell_{1:M}^S | \sigma^2 \sim \mathcal{N}\left( C\theta_{1:M}^{1:2} \begin{pmatrix} -2c\theta_* \\ \mathrm{vech}(c) \end{pmatrix}, \sigma^2 C W^{-1} C^\top + C\theta_{1:M} n K_1 \theta_{1:M}^\top C^\top \right)$$

where $C = (-\mathbf{1}_{M-1}, I_{M-1})$. In fact, since we are concerned about relative values of $\ell^S(\theta_m)$, $m \in 1:M$, we can use any $(M-1) \times M$ matrix $C$ whose rows are independent of each other and orthogonal to $(1, \dots, 1)$. It can be checked using the Sherman-Morrison-Woodbury formula $(A + BCD)^{-1} = A^{-1} - A^{-1}B(C^{-1} + DA^{-1}B)^{-1}DA^{-1}$ that

$$C^\top (CW^{-1}C^\top)^{-1} C = W - (\mathbf{1}_M^\top W \mathbf{1}_M)^{-1} W \mathbf{1}_M \mathbf{1}_M^\top W =: \overline{W}$$

[14]. We let

$$Q = (CW^{-1}C^\top + \sigma^{-2} C\theta_{1:M} n K_1 \theta_{1:M}^\top C^\top)^{-1}.$$

Then again by the Sherman-Morrison-Woodbury formula, we have

$$\begin{aligned}
Q &= (CW^{-1}C^\top)^{-1} \\
&\quad - (CW^{-1}C^\top)^{-1} C\theta_{1:M} \{\sigma^2 n^{-1} K_1^{-1} + \theta_{1:M}^\top C^\top (CW^{-1}C^\top)^{-1} C\theta_{1:M}\}^{-1} \theta_{1:M}^\top C^\top (CW^{-1}C^\top)^{-1}.
\end{aligned}$$

If we let $P = C^\top Q C$, we have

$$P = \overline{W} - \overline{W}\theta_{1:M}(\sigma^2 n^{-1} K_1^{-1} + \theta_{1:M}^\top \overline{W}\theta_{1:M})^{-1}\theta_{1:M}^\top \overline{W}.$$

We denote by $\hat{Q}$ the matrix obtained by substituting $\hat{\sigma}^2$ for $\sigma^2$ and $\hat{K}_1$ for $K_1$ in the expression for $Q$:

$$\begin{aligned}&\hat{Q} = (CW^{-1}C^\top)^{-1}\\ &- (CW^{-1}C^\top)^{-1}C\theta_{1:M}\{\hat{\sigma}^2 n^{-1}\hat{K}_1^{-1} + \theta_{1:M}^\top C^\top (CW^{-1}C^\top)^{-1}C\theta_{1:M}\}^{-1}\theta_{1:M}^\top C^\top (CW^{-1}C^\top)^{-1}.\end{aligned}$$

Then we have $\hat{P} = C^\top \hat{Q} C$.

The log density function of (26) evaluated at $C\ell_{1:M}^S$, or the marginal metamodel log-likelihood, is given by

$$\begin{aligned}\log p_{\text{meta}}(C\hat{\ell}_{1:M}^S|\theta_*, c, \sigma^2) = -\frac{M-1}{2}\log 2\pi - \frac{1}{2}\log\det(\sigma^2 Q^{-1})\\ - \frac{1}{2\sigma^2}\left\|\ell_{1:M}^S - \theta_{1:M}^{1:2}\begin{pmatrix}-2c\theta_*\\ \text{vech}(c)\end{pmatrix}\right\|_{C^\top QC}^2\end{aligned}$$

Using the matrix determinant lemma $\det(A+BCD) = \det(C^{-1} + DA^{-1}B)\det(A)\det(C)$, we see that

$$\begin{aligned}\det Q^{-1} &= \det\left\{CW^{-1}C^\top + \sigma^{-2}(C\theta_{1:M})nK_1(C\theta_{1:M})^\top\right\}\\ &= \det\left\{\sigma^2 n^{-1}K_1^{-1} + (C\theta_{1:M})^\top (CW^{-1}C^\top)^{-1}(C\theta_{1:M})\right\}\det(\sigma^{-2}nK_1)\det(CW^{-1}C^\top)\\ &= \det\left\{I_d + \sigma^{-2}nK_1\theta_{1:M}^\top \overline{W}\theta_{1:M}\right\}\det(CW^{-1}C^\top).\end{aligned}$$

Therefore, we have

$$\begin{aligned}\log p_{\text{meta}}(C\ell_{1:M}^S|\theta_*, c, \sigma^2) = \mathit{const.} - \frac{1}{2\sigma^2}\left\|\ell_{1:M}^S - \theta_{1:M}^{1:2}\begin{pmatrix}-2c\theta_*\\ \text{vech}(c)\end{pmatrix}\right\|_{C^\top QC}^2\\ - \frac{M-1}{2}\log\sigma^2 - \frac{1}{2}\log\det(I_d + \sigma^{-2}nK_1\theta_{1:M}^\top \overline{W}\theta_{1:M}).\end{aligned} \quad \text{(S25)}$$

We substitute $\hat{\sigma}^2$ for $\sigma^2$ and $\hat{K}_1$ for $K_1$ in the third term on the right hand side of the above equation and substitute $\hat{P}$ for $P = C^\top QC$. The estimating equation for $\hat{\theta}_*$ and $\hat{c}$, namely Equation (27), is then obtained by a usual weighted least square estimate for

$$\min_{\theta_*, c}\left\|\ell_{1:M}^S - \theta_{1:M}^{1:2}\begin{pmatrix}-2c\theta_*\\ \text{vech}(c)\end{pmatrix}\right\|_{\hat{P}}^2.$$

Consider a test on $\theta_*$, $c$, and $\sigma^2$,

$$H_0 : \theta_* = \theta_{*,0},\ c = c_0,\ \sigma^2 = \sigma_0^2, \qquad H_1 : \text{not } H_0$$

for some null values $\theta_{*,0}$, $c_0$, and $\sigma_0^2$. An approximate test for these hypotheses can be conducted by using the marginal metamodel log-likelihood (S25). The marginal metamodel log-likelihood ratio statistic for this test is given by

$$\mathit{MLLR}_{\theta_{*,0},c_0,\sigma_0^2} = -\frac{1}{2\sigma_0^2}\left\|\ell_{1:M}^S - \theta_{1:M}^{1:2}\begin{pmatrix}-2c_0\theta_{*,0}\\ \text{vech}(c_0)\end{pmatrix}\right\|_{\hat{P}}^2 + \frac{M-1}{2}\log\frac{\hat{\sigma}_{\text{2nd}}^2}{\sigma_0^2} + \frac{M-1}{2}, \quad \text{(S26)}$$

where $\hat{\sigma}_{\text{2nd}}^2$ is the second stage estimate given by (28). The distribution of the $\mathit{MLLR}_{\theta_{*,0},c_0,\sigma_0^2}$ statistic under $H_0 : \theta_* = \theta_{*,0}, c = c_0, \sigma^2 = \sigma_0^2$ is given by Proposition S6 at the end of this section.

A test on the simulation-based proxy $H_0 : \theta_* = \theta_{*,0},\ H_1 : \theta_* \neq \theta_{*,0}$ can be carried out by using the marginal metamodel log-likelihood ratio statistic obtained by taking the supremum of $\mathit{MLLR}_{\theta_{*,0},c_0,\sigma_0^2}$ over $c_0$ and $\sigma_0^2$:

$$\mathit{MLLR}_{\theta_{*,0}} = \sup_{c_0,\sigma_0^2}\mathit{MLLR}_{\theta_{*,0},c_0,\sigma_0^2}. \quad \text{(S27)}$$

*Proof of Proposition 5.* We consider the model

$$C\ell^S_{1:M} \sim \mathcal{N}\left(C\theta^{1:2}_{1:M}\begin{pmatrix}-2c\theta_* \\ \mathrm{vech}(c)\end{pmatrix}, \sigma^2\hat{Q}^{-1}\right),$$

where we use the plug-in estimate $\hat{Q}$ for the variance. Define a random vector $\mathbf{Z}$ such that

$$C\ell^S_{1:M} = C\theta^{1:2}_{1:M}\begin{pmatrix}-2c\theta_* \\ \mathrm{vech}(c)\end{pmatrix} + \sigma\hat{Q}^{-1/2}\mathbf{Z}, \tag{S28}$$

so that $\mathbf{Z} \sim \mathcal{N}(0, I_{M-1})$, approximately. We then have

$$\begin{aligned}\left(I_{M-1} - \hat{Q}^{1/2}C\theta^{1:2}_{1:M}\{{\theta^{1:2}_{1:M}}^\top C^\top\hat{Q}C\theta^{1:2}_{1:M}\}^{-1}\theta^{1:2}_{1:M}C^\top\hat{Q}^{1/2}\right)\hat{Q}^{1/2}C\ell^S_{1:M}& \\ = \left(I_{M-1} - \hat{Q}^{1/2}C\theta^{1:2}_{1:M}\{{\theta^{1:2}_{1:M}}^\top C^\top\hat{Q}C\theta^{1:2}_{1:M}\}^{-1}\theta^{1:2}_{1:M}C^\top\hat{Q}^{1/2}\right)\sigma\mathbf{Z}&\end{aligned} \tag{S29}$$

From (27) and (S29), we have

$$\begin{aligned}\hat{\sigma}^2_{\mathrm{2nd}} &= \frac{1}{M-1}\left\|\hat{Q}^{1/2}C\ell^S_{1:M} - n\hat{Q}^{1/2}C\theta^{1:2}_{1:M}\begin{pmatrix}-2\hat{c}\hat{\theta}_* \\ \mathrm{vech}(\hat{c})\end{pmatrix}\right\|^2 \\ &= \frac{1}{M-1}\left\|\left(I_{M-1} - \hat{Q}^{1/2}C\theta^{1:2}_{1:M}\{{\theta^{1:2}_{1:M}}^\top C^\top\hat{Q}C\theta^{1:2}_{1:M}\}^{-1}\theta^{1:2}_{1:M}C^\top\hat{Q}^{1/2}\right)\hat{Q}^{1/2}C\ell^S_{1:M}\right\|^2 \\ &= \frac{\sigma^2}{M-1}\mathbf{Z}^\top\left(I_{M-1} - \hat{Q}^{1/2}C\theta^{1:2}_{1:M}\{{\theta^{1:2}_{1:M}}^\top C^\top\hat{Q}C\theta^{1:2}_{1:M}\}^{-1}\theta^{1:2}_{1:M}C^\top\hat{Q}^{1/2}\right)\mathbf{Z} \\ &\sim \frac{\sigma^2}{M-1}\chi^2_{M-\frac{d^2+3d+2}{2}},\end{aligned}$$

since $\hat{Q}^{1/2}C\theta^{1:2}_{1:M} \in \mathbb{R}^{(M-1)\times\frac{d^2+3d}{2}}$ is a rank $\frac{d^2+3d}{2}$ matrix.

Now suppose that the null hypothesis $H_0 : \theta_* = \theta_{*,0}$ is true. Then by the usual results for weighted least squares regression, we have

$$\begin{aligned}&\inf_c\left\|\hat{Q}^{1/2}C\ell^S_{1:M} - \hat{Q}^{1:2}C\theta^{1:2}_{1:M}\begin{pmatrix}-2c\theta_{*,0} \\ \mathrm{vech}(c)\end{pmatrix}\right\|^2 \\ &\qquad= \inf_{K_2}\left\|\hat{Q}^{1/2}C\ell^S_{1:M} - \hat{Q}^{1:2}C\theta^{1:2}_{1:M}\begin{pmatrix}-\theta_{*,0,\mathrm{mat}} \\ -\frac{1}{2}I_{\frac{d^2+d}{2}}\end{pmatrix}n\mathrm{vech}(K_2)\right\|^2 \\ &\qquad= \inf_{K_2}\left\|\ell^S_{1:M} - T(\theta_{*,0})n\mathrm{vech}(K_2)\right\|^2_{\hat{P}} \\ &\qquad= \left\|\left(I_{M-1} - T(\theta_{*,0})\{T(\theta_{*,0})^\top\hat{P}T(\theta_{*,0})\}^{-1}T(\theta_{*,0})^\top\hat{P}\right)\ell^S_{1:M}\right\|^2_{\hat{P}} \\ &\qquad= \left\|\{I_{M-1} - S(\theta_{*,0})\hat{P}\}\ell^S_{1:M}\right\|^2_{\hat{P}}\end{aligned}$$

Since the maximum of $-\frac{a}{x} - b\log x$ over $x > 0$ is obtained at $x = a/b$ for $a, b > 0$, we have

$$\begin{aligned}MLLR_{\theta_{*,0}} &= \sup_{\sigma_0^2} -\frac{1}{2\sigma_0^2}\left\|\{I_{M-1} - S(\theta_{*,0})\hat{P}\}\ell^S_{1:M}\right\|^2_{\hat{P}} + \frac{M-1}{2}\log\frac{\hat{\sigma}^2_{\mathrm{2nd}}}{\sigma_0^2} + \frac{M-1}{2} \\ &= -\frac{M-1}{2} + \frac{M-1}{2}\log\frac{(M-1)\hat{\sigma}^2_{\mathrm{2nd}}}{\left\|\{I_{M-1} - S(\theta_{*,0})\hat{P}\}\ell^S_{1:M}\right\|^2_{\hat{P}}} + \frac{M-1}{2} \\ &= -\frac{M-1}{2}\log\frac{\left\|\{I_{M-1} - S(\theta_{*,0})\hat{P}\}\ell^S_{1:M}\right\|^2_{\hat{P}}}{(M-1)\hat{\sigma}^2_{\mathrm{2nd}}}.\end{aligned}$$

Let

$$H := \hat{Q}^{1/2} C \theta_{1:M}^{1:2} ({\theta_{1:M}^{1:2}}^\top C^\top \hat{Q} C \theta_{1:M}^{1:2})^{-1} {\theta_{1:M}^{1:2}}^\top C^\top \hat{Q}^{1/2} \tag{S30}$$

be a orthogonal projection matrix of rank $\frac{d^2+3d}{2}$ and

$$G := \hat{Q}^{1/2} C T(\theta_{*,0}) \left\{ T(\theta_{*,0})^\top \hat{P} T(\theta_{*,0}) \right\}^{-1} T(\theta_{*,0})^\top C^\top \hat{Q}^{1/2}$$

be another orthogonal projection matrix of rank $\frac{d^2+d}{2}$. We have $GH = HG = G$, that is, $G$ is a nested orthogonal projection with respect to $H$. We have

$$(I - G)\hat{Q}^{1/2} C \ell_{1:M}^S = (I - G)\sigma \mathbf{Z}$$

due to (S29). Thus we obtain

$$\|(I - G)\hat{Q}^{1/2} C \ell_{1:M}^S\|^2 = \sigma^2 \mathbf{Z}^\top (I - G)\mathbf{Z} = (M-1)\hat{\sigma}_{\text{2nd}}^2 + \sigma^2 \mathbf{Z}^\top (H - G)\mathbf{Z}. \tag{S31}$$

Since $H - G$ is an orthogonal projection matrix with rank $\frac{d^2+3d}{2} - \frac{d^2+d}{2} = d$, we have

$$\|(I - G)\hat{Q}^{1/2} C \ell_{1:M}^S\|^2 - (M-1)\hat{\sigma}_{\text{2nd}}^2 = \mathbf{Z}^\top (H - G)\mathbf{Z} \sim \sigma^2 \chi_d^2,$$

and since $(I - H)(H - G) = 0$, we have that the above display and $(M-1)\hat{\sigma}_{\text{2nd}}^2 \sim \sigma^2 \chi^2_{M - \frac{d^2+3d+2}{2}}$ are independent. It follows that

$$\begin{aligned}
\frac{\|\{I_{M-1} - S(\theta_{*,0})\hat{P}\}\ell_{1:M}^S\|_{\hat{P}}^2}{(M-1)\hat{\sigma}_{\text{2nd}}^2} - 1 &= \frac{\|(I - G)\hat{Q}^{1/2} C \ell_{1:M}^S\|^2}{(M-1)\hat{\sigma}_{\text{2nd}}^2} - 1 \\
&= \frac{\sigma^2 \mathbf{Z}^\top (I - G)\mathbf{Z}}{\sigma^2 \mathbf{Z}^\top (I - H)\mathbf{Z}} - 1 \\
&= \frac{\mathbf{Z}^\top (H - G)\mathbf{Z}}{\mathbf{Z}^\top (I - H)\mathbf{Z}} \\
&\sim \frac{\chi_d^2}{\chi^2_{M - \frac{d^2+3d+2}{2}}} \\
&= \frac{d}{M - \frac{d^2+3d+2}{2}} F_{d, M - \frac{d^2+3d+2}{2}}.
\end{aligned}$$

□

One might be concerned about the fact the test is based on the distribution (26) that is conditioned on $\sigma^2$. However, since the distribution of the test statistic (29) under $H_0$ does not depend on the value of $\sigma^2(Y_{1:n})$, its marginal distribution over $\sigma^2(Y_{1:n})$ is the same. Therefore, the test is valid nonetheless. The same reasoning was used by Zellner [15] to consider multivariate $t$-distributed errors in linear regression.

*Proof of Corollary 2.* We have

$$\begin{aligned}
&\|\{I_{M-1} - S(\theta_{*,0})\hat{P}\}\ell_{1:M}^S\|_{\hat{P}}^2 \\
&= {\ell_{1:M}^S}^\top \left( \hat{P} - \hat{P} S(\theta_{*,0}) \hat{P} \right) \ell_{1:M}^S \\
&= \|\ell_{1:M}^S\|_{\hat{P}}^2 - {\ell_{1:M}^S}^\top \hat{P} \theta_{1:M}^{1:2} \begin{pmatrix} \theta_0 \\ -\frac{1}{2} \end{pmatrix} \left\{ (\theta_0, -\frac{1}{2}) {\theta_{1:M}^{1:2}}^\top \hat{P} \theta_{1:M}^{1:2} \begin{pmatrix} \theta_0 \\ -\frac{1}{2} \end{pmatrix} \right\}^{-1} (\theta_0, -\frac{1}{2}) {\theta_{1:M}^{1:2}}^\top \hat{P} \ell_{1:M}^S \\
&= \|\ell_{1:M}^S\|_{\hat{P}}^2 - \frac{(\zeta_1 \theta_0 - \frac{1}{2}\zeta_2)^2}{\rho_{11}\theta_0^2 - \rho_{12}\theta_0 + \frac{1}{4}\rho_{22}}.
\end{aligned}$$

The null $H_0 : \theta = \theta_0$ is not rejected at an approximate significance level $\alpha$ if

$$\|\{I_{M-1} - S(\theta_{*,0})\hat{P}\}\ell_{1:M}^S\|_{\hat{P}}^2 < (M-1)\hat{\sigma}_{\text{2nd}}^2 \left( \frac{F_{1, M-3, \alpha}}{M-3} + 1 \right).$$

This is equivalent to

$$\|\ell^S_{1:M}\|^2_{\hat{P}} - (M-1)\hat{\sigma}^2_{\mathrm{2nd}}\left(\frac{F_{1,M-3,\alpha}}{M-3}+1\right) < \frac{(\zeta_1\theta_0 - \frac{1}{2}\zeta_2)^2}{\rho_{11}\theta_0^2 - \rho_{12}\theta_0 + \frac{1}{4}\rho_{22}}.$$

Denoting the left hand side of the above inequality by $\zeta_0$, we can rearrange the terms to obtain

$$(\zeta_0\rho_{11} - \zeta_1^2)\theta_0^2 + (\zeta_1\zeta_2 - \zeta_0\rho_{12})\theta_0 + \frac{1}{4}(\rho_{22}\zeta_0 - \zeta_2^2) < 0,$$

which gives an approximate level $1-\alpha$ confidence interval for $\theta$. □

We conclude this section by giving the null distribution of the $MLLR_{\theta_{*,0},c_0,\sigma_0^2}$ statistic as follows.

**Proposition S6.** *Suppose that Assumptions 1-6 hold. If $Q = \hat{Q}$, then the $MLLR_{\theta_{*,0},c_0,\sigma_0^2}$ statistic under $H_0 : \theta_* = \theta_{*,0}, c = c_0, \sigma^2 = \sigma_0^2$ follows the $\mathsf{SCL}(M-1, \frac{d^2+3d}{2})$ distribution.*

*Proof of Proposition S6.* From (S26) and (S28), we have

$$MLLR_{\theta_{*,0},c_0,\sigma_0^2} = -\frac{1}{2}\|\mathbf{Z}\|^2 + \frac{M-1}{2}\log\frac{\mathbf{Z}^\top(I_{M-1}-H)\mathbf{Z}}{M-1} + \frac{M-1}{2}$$

where $H$ is defined by (S30). In the proof of Proposition 5, we showed that

$$X_1 := \mathbf{Z}^\top H\mathbf{Z} \sim \chi^2_{\frac{d^2+3d}{2}}, \quad X_2 := \mathbf{Z}^\top(I_{M-1}-H)\mathbf{Z} \sim \chi^2_{M-\frac{d^2+3d+2}{2}}$$

and that $X_1$ and $X_2$ are independent. Therefore, the $MLLR_{\theta_{*,0},c_0,\sigma_0^2}$ statistic follows the $\mathsf{SCL}(M-1, \frac{d^2+3d}{2})$ distribution. □

# S6 Monte Carlo correction of the bias in the test on $\theta_*$

Our hypothesis testing procedure for the simulation-based proxy uses a plug-in estimate $\hat{K}_1$ of $K_1$. The estimation error in $\hat{K}_1$ introduces a bias in the test. This bias may be reduced by a Monte Carlo method that takes into account the variability in $\hat{K}_1$, described as follows. The test statistic for the test on $\theta_*$ is given by (29),

$$\frac{M - \frac{d^2+3d+2}{2}}{d}\left\{\frac{\|\{I_{M-1} - S(\theta_{*,0})\hat{P}\}\ell^S_{1:M}\|^2_{\hat{P}}}{(M-1)\hat{\sigma}^2_{\mathrm{2nd}}} - 1\right\}.$$

In order to obtain a Monte Carlo draw for the test statistic, we regard the estimated $\hat{K}_1$, $\hat{\sigma}^2_{\mathrm{2nd}}$, and $\hat{\theta}_*$ as if they are equal to the true values. We first create a Monte Carlo simulation for the vector $\ell^S_{1:M}$. From (S28), we see that a Monte Carlo simulation $\ell^S_{1:M,MC}$ can be obtained via

$$\hat{Q}^{1/2}C\ell^S_{1:M,MC} = \hat{Q}^{1/2}C\theta^{1:2}_{1:M}\begin{pmatrix}-2\hat{c}\hat{\theta}_*\\ \mathrm{vech}(\hat{c})\end{pmatrix} + \hat{\sigma}_{\mathrm{2nd}}\mathbf{Z}_{MC}$$

where $\mathbf{Z}_{MC}$ is a random draw from $\mathcal{N}(0, I_{M-1})$. Here $\hat{\theta}_*$ and $\mathrm{vech}(\hat{c})$ are the point estimates obtained by (27). Since $\hat{Q}$ is invertible and the left multiplication of $\ell^S_{1:M,MC}$ by $C$ gives relative values with respect to $\ell^S_{1,MC}$, we can let without loss of generality

$$\ell^S_{1,MC} := 0, \qquad \ell^S_{2:M,MC} = \hat{Q}^{-1/2}\left\{\hat{Q}^{1/2}C\theta^{1:2}_{1:M}\begin{pmatrix}-2\hat{c}\hat{\theta}_*\\ \mathrm{vech}(\hat{c})\end{pmatrix} + \hat{\sigma}_{\mathrm{2nd}}\mathbf{Z}_{MC}\right\}.$$

A Monte Carlo draw for the first stage estimate of $\sigma^2$ is given by

$$\sigma^2_{MC} := \frac{1}{M}\|(I - \theta^{0:2}_{1:M}\{\theta^{0:2}_{1:M}{}^\top W\theta^{0:2}_{1:M}\}^{-1}\theta^{0:2}_{1:M}{}^\top W)\ell^S_{1:M,MC}\|^2.$$

Denote by $\tau_1$ and $\tau_2$ the first and the second term on the right hand side of (22), which is used to obtain an estimate $\hat{K}_1$. If $Y_{1:n}$ are iid and $\tau_1$ is estimated by the sample variance of the $n$ estimated slopes of the fitted quadratic polynomial, a Monte Carlo draw $\tau_{1,MC}$ can be obtained by a draw from the Wishart distribution $\mathcal{W}_d(\frac{1}{\nu}\tau_1, \nu)$ where the degrees of freedom is equal to $\nu = n - 1$. If $\tau_1$ is estimated by using $n_b$ batch estimates, a Monte Carlo draw is obtained from $\mathcal{W}_d(\frac{1}{\nu}\tau_1, \nu)$ with $\nu = n_b - 1$. A Monte Carlo draw for $\tau_2$ is obtained by

$$\tau_{2,MC} = \frac{1}{n}(\mathbf{0}_d, I_d, 2\theta_{\mathrm{mat}})(\theta_{1:M}^{0:2\,\top} W \theta_{1:M}^{0:2})^{-1}(\mathbf{0}_d, I_d, 2\theta_{\mathrm{mat}})^\top \hat{\sigma}^2_{MC}$$

(see (23).) A Monte Carlo draw for $\hat{K}_1$ is then obtained by

$$\hat{K}_{1,MC} = \tau_{1,MC} - \tau_{2,MC}.$$

A Monte Carlo replicate for $\hat{Q}$ is given by

$$\hat{Q}_{MC} := \{CW^{-1}C^\top + \sigma_{MC}^{-2} C\theta_{1:M} n \hat{K}_{1,MC} \theta_{1:M}^\top C^\top\}^{-1}.$$

We let $\hat{P}_{MC} := C^\top \hat{Q}_{MC} C$. A Monte Carlo draw for the second stage estimate $\hat{\sigma}^2_{\mathrm{2nd}}$ is obtained by

$$\hat{\sigma}^2_{\mathrm{2nd},MC} = \frac{1}{M-1} \left\| \ell^S_{1:M,MC} - \theta^{1:2}_{1:M} \left\{ \theta^{1:2\,\top}_{1:M} \hat{P}_{MC} \theta^{1:2}_{1:M} \right\}^{-1} \theta^{1:2\,\top}_{1:M} \hat{P}_{MC} \ell^S_{1:M,MC} \right\|^2_{\hat{P}_{MC}}.$$

If we write

$$S(\hat{\theta}_*) = T(\hat{\theta}_*)\{T(\hat{\theta}_*)^\top \hat{P}_{MC} T(\hat{\theta}_*)\}^{-1} T(\hat{\theta}_*)^\top$$

where $T(\hat{\theta}_*) = \theta^{1:2}_{1:M} \begin{pmatrix} \hat{\theta}_{*,\mathrm{mat}} \\ -\frac{1}{2} I_{\frac{d^2+d}{2}} \end{pmatrix}$, a Monte Carlo draw for the test statistic is then given by

$$\frac{M - \frac{d^2+3d+2}{2}}{d} \left\{ \frac{\|\{I_{M-1} - S(\hat{\theta}_*)\hat{P}_{MC}\}\ell^S_{1:M,MC}\|^2_{\hat{P}_{MC}}}{(M-1)\hat{\sigma}^2_{\mathrm{2nd},MC}} - 1 \right\}.$$

A Monte Carlo corrected p-value for the hypothesis test on $\theta_*$ can be found by using the empirical distribution of the replicated Monte Carlo draws in place of the $F_{d, M-\frac{d^2+3d+2}{2}}$ distribution in (29).

# S7 Additional numerical results

## S7.1 Additional figures for the gamma-Poisson example in Section 5.1

Here we provide additional figures for the gamma-Poisson example considered in Section 5.1. Figure S-1 shows the distributions of the p-value for the hypothesis test $H_0 : \lambda_{MESLE} = \lambda_{MESLE,0}$, $H_1 : \lambda_{MESLE} \neq \lambda_{MESLE,0}$ for varied null values $\lambda_{MESLE,0}$. The distribution of the p-value when the null value $\lambda_{MESLE,0}$ equals the exact MESLE is close to the uniform distribution, indicating that our estimation and uncertainty quantification method for the MESLE has little bias. The other two plots in Figure S-1 show that the p-values are skewed toward zero when the null value is not equal to the exact MESLE, indicating that the power is greater than the significance level.

Figure S-2 shows the distribution of the p-value for the test on the third order term in the Taylor expansion of $\mu(\theta; y_{1:n})$ mentioned at the end of Section 4. The distribution of the p-value is close to uniform, indicating that the quadratic approximation of $\mu(\theta; y_{1:n})$ was adequate. If the simulation points were taken from a wider range, this distribution would be skewed toward zero.

Figure S-3 shows the distributions of the p-values for hypothesis tests for the simulation-based proxy, $H_0 : \lambda_* = \lambda_{*,0}$, $H_1 : \lambda_* \neq \lambda_{*,0}$ for varied null values $\lambda_{*,0}$. The left plot shows that the proportion of the replications where the p-value is between 0 and 0.05 is somewhat greater than what would be expected under the uniform distribution, implying the presence of some bias in the test. For $\lambda_{*,0} = 0.9$, the p-values are skewed toward zero, indicating a reasonably high power. The empirical probability of rejecting the null hypothesis shown in Figure 5 was minimized at $\lambda_{*,0} = 1.025$. For this null value, the distribution of the p-value was close to uniform, as shown by the right plot of S-3. Although this implies a bias in estimating the true value of $\lambda_0 = 1$, the magnitude ($\approx 0.025$) is not large.

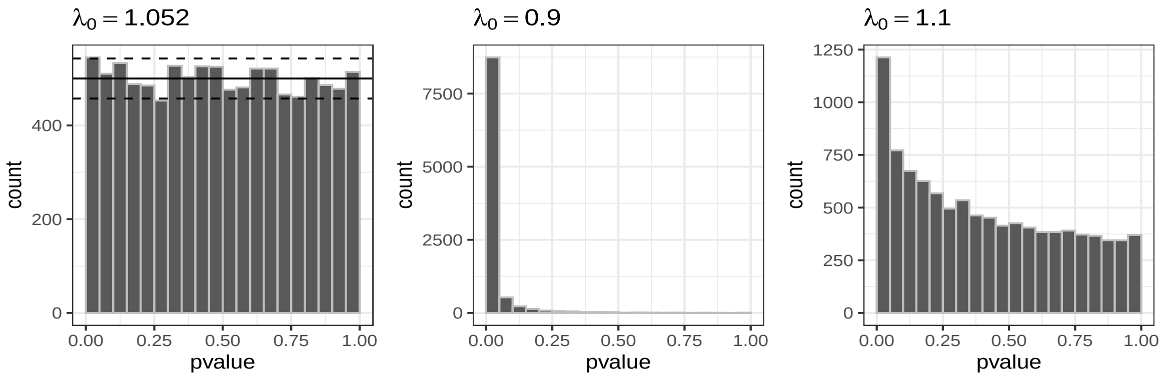


Figure S-1: The distribution of the p-value for the test on the MESLE for varied null values. The horizontal lines on the left plot show the expected counts under the uniform distribution (solid) and 95% confidence bounds (dashed).

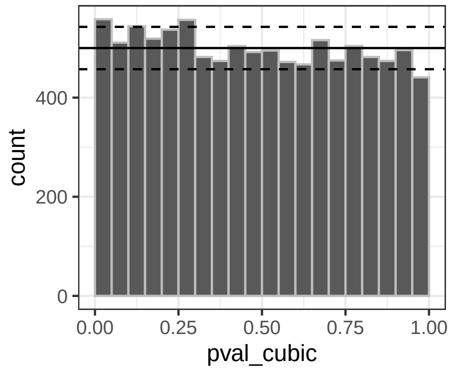


Figure S-2: The distribution of the p-value for the test on the cubic coefficient for the expected simulated log-likelihood.

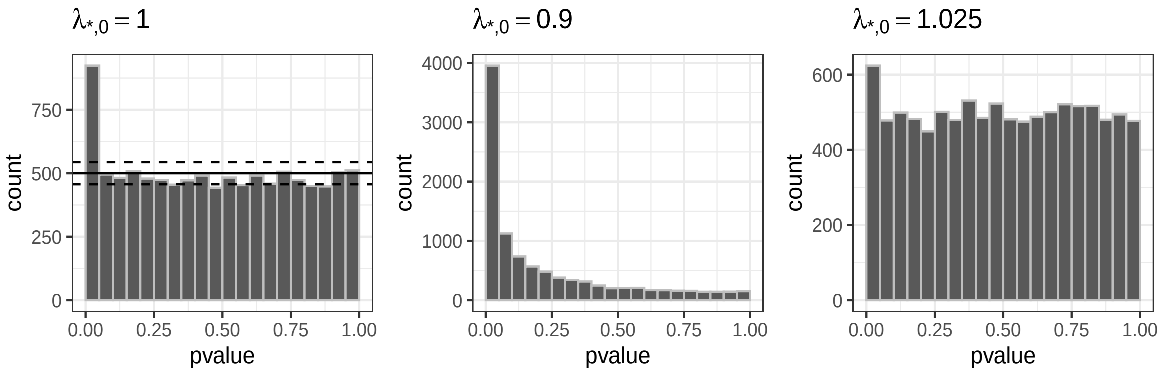


Figure S-3: Distribution of the p-values for the test on the simulation-based proxy $\lambda_*$ for varied null values $\lambda_{*,0}$.

## S7.2 Normal processes with normally distributed observations

Here we show numerical results for an example not considered in the main text. Example S2 describes a normal process $X_{1:n} \overset{iid}{\sim} \mathcal{N}(\theta, I_2)$ observed with $\mathcal{N}(0, I_2)$-distributed noises. The mean parameter $\theta \in \mathbb{R}^2$ is estimated using simulations. We generated $n = 1000$ observations at $\theta_0 = (1, 1)$. The MESLE is given by the sample mean of observations, $\theta_{MESLE} = \bar{y} = \frac{1}{n}\sum_{i=1}^{n} y_i \in \mathbb{R}^2$. Simulations are carried out at $(\theta_1, \theta_2) = (1 \pm 0.02 \times k_1, 1 \pm 0.02 \times k_2)$ where $k_1, k_2 \in 0:10$.

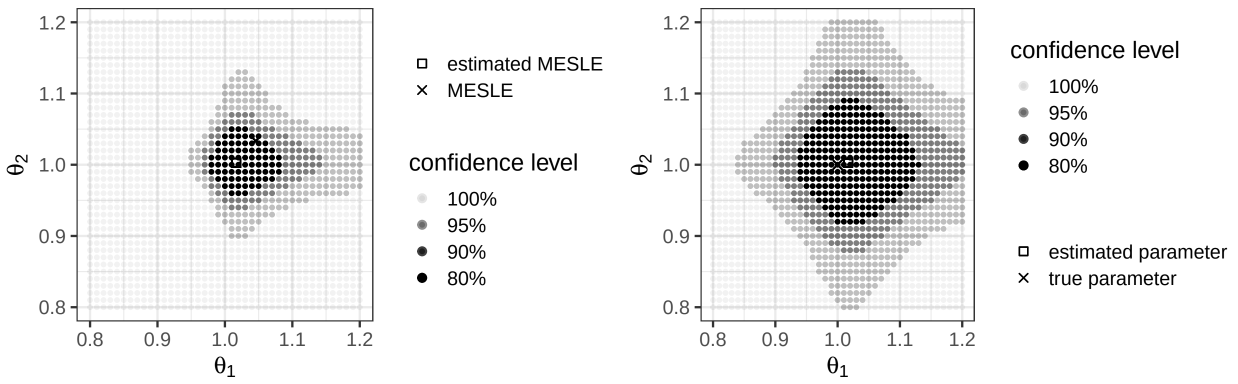


Figure S-4: Left: Constructed confidence regions for $\theta_{MESLE}$. Right: Constructed confidence regions for $\theta_*$.

Tests on the MESLE, $H_0 : \theta_{MESLE} = \theta_{MESLE,0}$, $H_1 : \theta_{MESLE} \neq \theta_{MESLE,0}$ were carried out. A $100(1-\alpha)\%$ confidence region for $\theta_{MESLE}$ can be obtained by collecting all null values for which the p-value is greater than $\alpha$. The left plot in Figure S-4 shows the constructed confidence regions for $\theta_{MESLE}$. Similarly, tests on the simulation-based parameter proxy $H_0 : \theta_* = \theta_{*,0}$, $H_1 : \theta_* \neq \theta_{*,0}$ were conducted, and confidence regions were constructed. The constructed confidence regions for $\theta_*$ are shown in the right plot of Figure S-4.

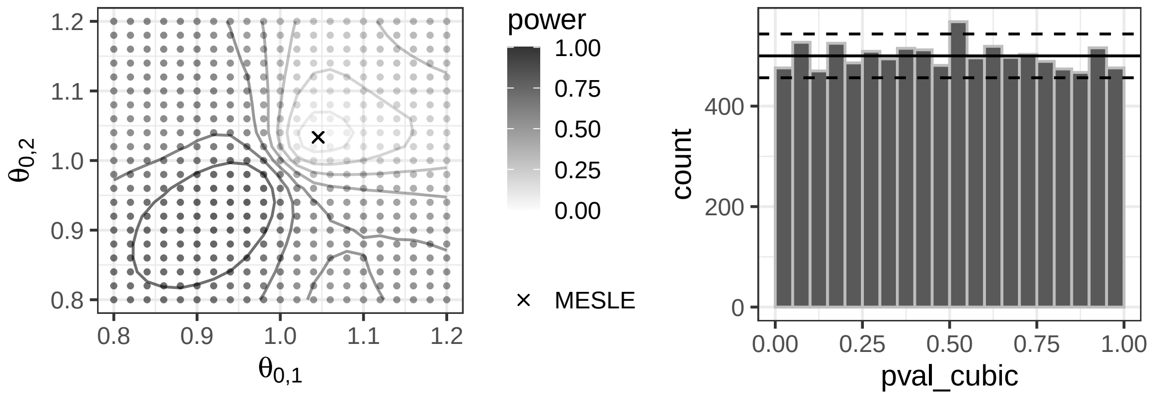


Figure S-5: Left: Probability of rejecting $H_0 : \theta_{MESLE} = \theta_{MESLE,0}$ at a 5% significance level, where the contours show the level sets. Right: Distribution of p-values for the test on the cubic coefficient for the expected simulated log-likelihood function.

We replicated hypothesis test $H_0 : \theta_{MESLE} = \theta_{MESLE,0}$ for varied null values 10000 times. The left plot of Figure S-5 shows the probabilities of rejecting the null hypothesis for varied null values $\theta_{MESLE,0}$. The right plot of Figure S-5 shows the distribution of the p-values for the test on significance of the third-order term in the Taylor expansion of $\mu(\theta)$. The distribution of the p-values for the cubic test is close to uniform, implying that the range of simulation points were suitably chosen.

We carried out hypothesis tests on the simulation-based proxy, which is the same as the true parameter value $\theta = (1, 1)$ for this example. For each of 10000 replications, a new set of observations were generated under $\theta = (1, 1)$. The distribution of the p-value under the true null hypothesis $H_0 : \theta_* = \theta_{*,0} = (1, 1)$ is

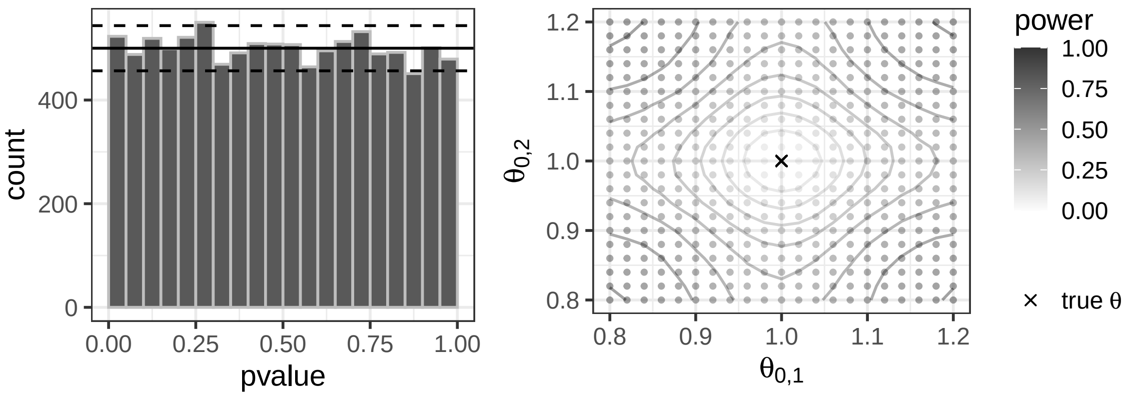


Figure S-6: Left: Distribution of the p-value for the test on the simulation-based proxy under a true null hypothesis, $H_0 : \theta_* = (1, 1)$. Right: Probability of rejecting the null hypothesis at a 5% significance level for varied null values. The contours show the level sets.

shown in the left plot of Figure S-6. The distribution was close to uniform, implying that our test had little bias. The estimated probabilities of rejecting the null hypotheses at a 5% significance level for varied null values are shown in the right plot of Figure S-6.

### S7.3 Additional details and figures for the compartment model for the population dynamics of measles transmission in Section 5.3

We provide additional information about the SEIR model considered in Section 5.3 and additional numerical results. The population size at time $t$, $N(t)$, which is assumed to be known, is equal to the sum of $S(t)$, $E(t)$, $I(t)$, and $R(t)$, the compartment sizes at $t$. The compartment sizes evolve over time according to the stochastic equations (S32). The evolution of compartment sizes is described by the following stochastic equation:

$$\begin{aligned}
\mathrm{d}S(t) &= -\left\{\left(\frac{R_0 s(t)(I(t)+\iota)^\alpha}{N(t)} + \mu\right) S(t)\,\mathrm{d}t + \mathrm{d}W_{SE}(t) + \mathrm{d}W_{SD}(t)\right\} + \mathrm{d}b(t) \\
\mathrm{d}E(t) &= \left\{\frac{R_0 s(t)(I+\iota)^\alpha}{N(t)} S(t)\,\mathrm{d}t + \mathrm{d}W_{SE}(t)\right\} - \{(\gamma_{EI}+\mu)E(t)\,\mathrm{d}t + \mathrm{d}W_{EI}(t) + \mathrm{d}W_{ED}(t)\} \\
\mathrm{d}I(t) &= \{\gamma_{EI}\,\mathrm{d}t + \mathrm{d}W_{EI}(t)\} - \{(\gamma_{IR}+\mu)I(t)\,\mathrm{d}t + \mathrm{d}W_{IR}(t) + \mathrm{d}W_{ID}(t)\}.
\end{aligned} \tag{S32}$$

Here $b(t)$ is the cumulative number of entry into the S compartment (i.e., births), $R_0$ the basic reproduction number, $s(t)$ the seasonal fluctuation of the transmission rate, $\iota$ the number of infectious individuals visiting the population, $\alpha$ a mixing parameter, which is close to the unity, $\mu$ the mortality rate, $\gamma_{EI}$ and $\gamma_{IR}$ the rates of progression from E to I and from I to R respectively, $W_{**}$ the cumulative stochastic noises for transitions between compartments, where D signifies mortality. Each noise process $W_{**}(t)$ is modelled by a Poisson process subordinated by a gamma process, and its rate depends on the current compartment sizes. A fraction of cumulative transitions from I to R each week is assumed to be reported and recorded, with mean reporting rate $\rho$ and inflated variance relative to the binomial distribution. The variation inflation parameter is denoted by $\psi$.

In addition to the basic reproduction number $R_0$ (Figure 8), we carried out parameter inference for $\alpha$, a mixing parameter, and $\gamma_{EI}$ and $\gamma_{IR}$ the rates of progression from E to I and from I to R respectively. Partial observations of the compartment sizes are given by weekly reported case numbers, which are random fractions of weekly aggregate transitions from the infectious to the recovered compartment.

Unbiased likelihood estimate for the observed data sequence were obtained for varied parameters using the bootstrap particle filter via the `R` package `pomp`. The package vignette (`https://kingaa.github.io/pomp/vignettes/He2010.html`) describes steps for analyzing the observed data for London.

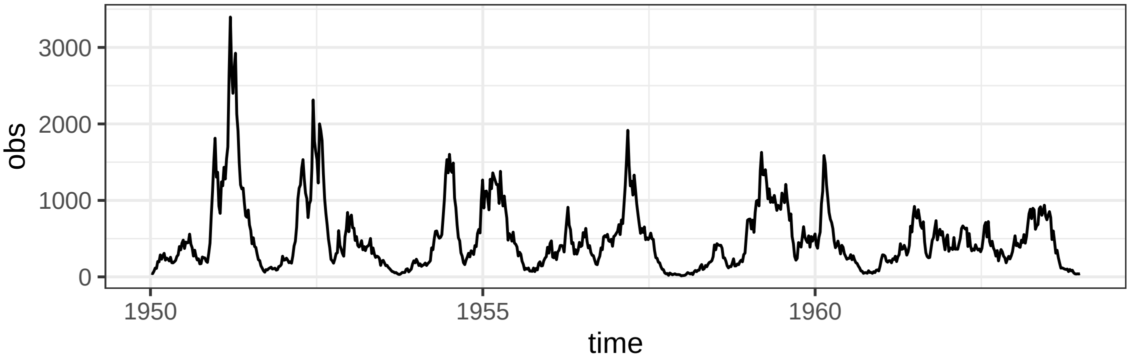


Figure S-7: A sequence of weekly reported measles cases generated by simulating the stochastic SEIR process for the chosen parameter vector.

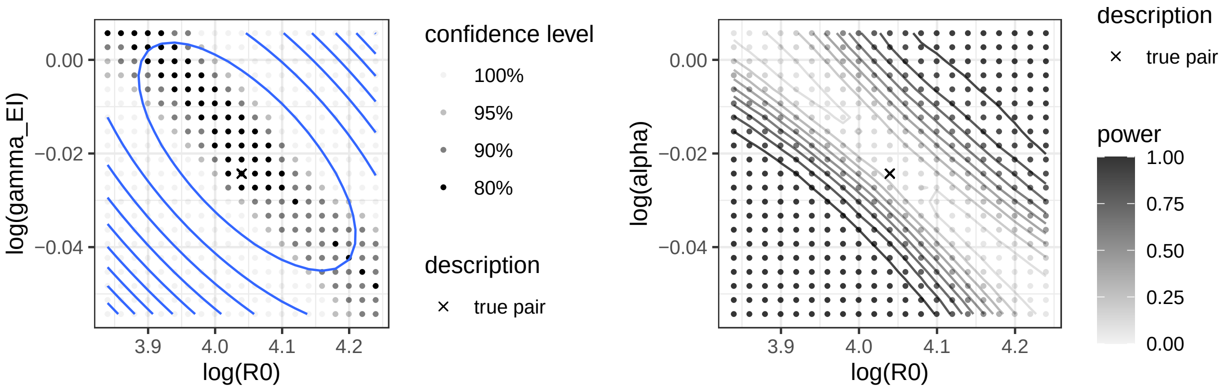


Figure S-8: Left: Constructed confidence regions for $R_0$ and $\alpha$. The contours show the level sets of the estimated expected simulated log-likelihood, $\hat{\mu}(\theta; y_{1:n})$. Right: Probabilities of rejecting the null hypothesis for varying null values at a 5% significance level. The contours show the level sets of the estimated rejection probabilities.

We simulated the SEIR model at a suitably chosen parameter vector and generated a sequence of weekly reported cases data. Since all considered parameters had positivity constraints, they were estimated on the log scale. The left plot of Figure 8 shows the simulated log-likelihoods for varying $\log(R_0)$, and the constructed 90% and 95% confidence intervals. Simulations were carried out at $M = 100$ points uniformly placed between the exact value $\pm 0.1$ on the log scale. We replicated hypothesis tests for $R_0$ 1000 times. The right plot of Figure 8 shows the probability of rejecting the null hypothesis at a 5% significance level for varying null values for $\log(R_0)$. The power at the true parameter value, indicated by the vertical dashed line, is about 10%, which is somewhat higher than the significance level, implying that there is a bias in our hypothesis test method. However, the rejection probability is closest to the significance level near the true parameter value.

Next we carried out hypothesis tests for pairs of the parameters among $R_0$, $\alpha$, $\gamma_{EI}$, and $\gamma_{IR}$. The constructed two dimensional confidence regions visualize the joint parameter inference. We note that all two dimensional slices of the mean function $\mu(\theta; y_{1:n})$ fully describe the local dependence of $\mu(\theta; y_{1:n})$ on the four parameters, because the mean function in our metamodel is locally quadratic. The left plot of Figure S-8 shows the constructed 80%, 90%, and 95% confidence regions for $R_0$ and $\alpha$ by marking the points where the p-value was higher than 20%, 10%, and 5%, respectively for the test on the pair of simulation-based proxy. Simulations were carried out at $M = 400$ points uniformly placed on the rectangle centered at the true value pair and having widths 0.2 for $\log(R_0)$ and 0.03 for $\log(\alpha)$. The elliptic contours on the plot show the level sets of the estimated expected simultion log-likelihood, $\hat{\mu}(\theta; y_{1:n})$. The p-value for the test on the

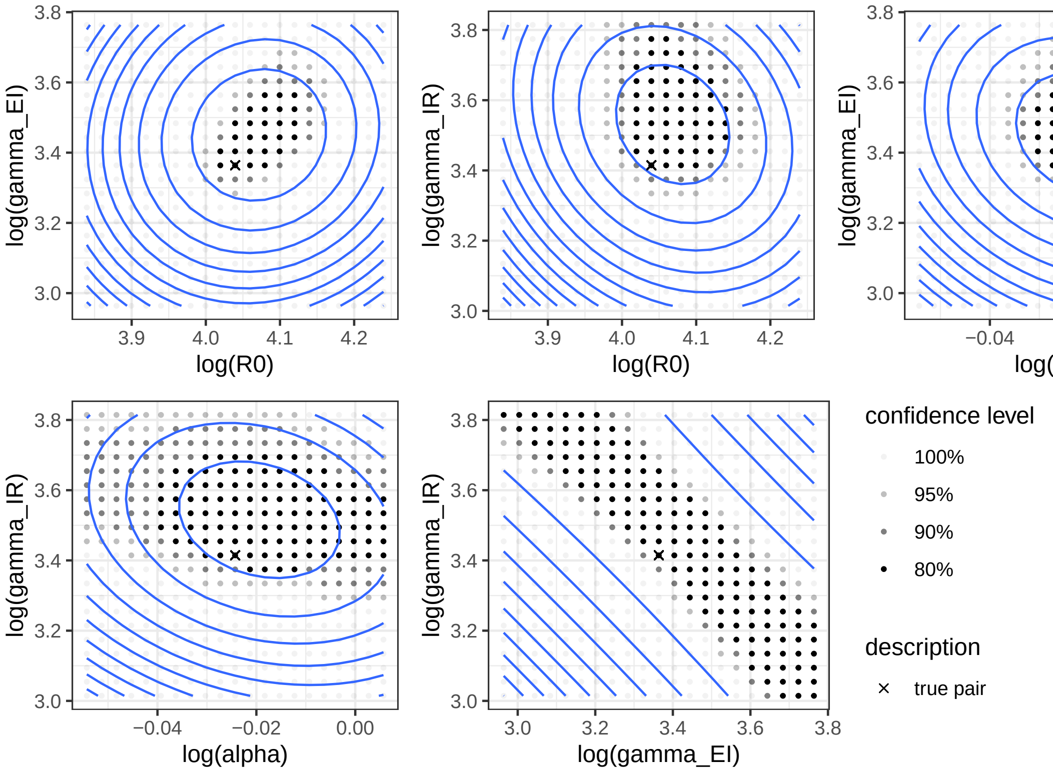


Figure S-9: Constructed confidence regions for pairs of parameters for the SEIR model. The contours show the level sets of the estimated expected simulated log-likelihood, $\hat{\mu}(\theta; y_{1:n})$.

significance of the cubic term in the expected simulated log-likelihood was 0.56, implying that the simulation points were appropriately chosen. These result show that $R_0$ and $\alpha$ are hardly identifiable jointly, unless a much longer observation sequence is analyzed. The statistical power could increase with more simulations (i.e., larger $M$) or with a greater range for simulation points. However, when we used simulation points from a wider range, the p-value for the test on the cubic coefficient in the mean function dropped close to zero, implying an increase in the bias in the test. Figure S-9 shows the constructed confidence regions for other pairs of parameters. These results show that all pairs except $(\alpha, R_0)$ and $(\gamma_{EI}, \gamma_{IR})$ can be jointly identified. The right plot of Figure S-8 shows the estimated probabilities of rejecting the null hypothesis for varying null values of the pair $\log(R_0)$ and $\log(\alpha)$ at a 5% significance level when the tests were repeated 1000 times.

# S8 Additional information on Section 6

## S8.1 Justification of the fact that the Monte Carlo standard error for pseudo-marginal MCMC is $\varnothing((\log M)^{-1/4})$

We justify below the claim made in Section 6 that the standard error of the estimates obtained by pseudo-marginal MCMC scales as $\varnothing((\log M)^{-1/4})$ where $M$ is the length of the constructed Markov chain. Suppose that initial state of the chain is denoted by $\theta_1$ and subsequent proposed values are denoted by $\theta_2, \ldots, \theta_M$. For simplicity, we will suppose that the acceptance probability for $\theta'$ given a current state $\theta$ is approximately given by

$$\min\left(1, \frac{\hat{L}(\theta'; y_{1:n})}{\hat{L}(\theta; y_{1:n})}\right) = \exp[-\{\ell^S(\theta) - \ell^S(\theta')\}_+] \qquad \text{where } a_+ := \max(a, 0)$$

by assuming that the log ratio $\left|\frac{h(\theta')q(\theta|\theta')}{h(\theta)q(\theta'|\theta)}\right|$ is small compared to the difference in $\ell^S$. We suppose that $\ell^S(\theta) = \log \hat{L}(\theta; y_{1:n})$ is normally distributed such that we can write

$$\ell^S(\theta_m) = \mu(\theta_m) + \sigma Z_m, \quad Z_m \overset{iid}{\sim} \mathcal{N}(0,1), \quad m \in 1\!:\!M$$

and that $\mu(\theta) = \text{const.} + (\theta - \theta_{MESLE})^\top c(\theta - \theta_{MESLE})$.

A candidate $\theta_m$ has a high chance to be accepted if $\mu(\theta_m) + \sigma Z_m$ is relatively large among other values. Denote the ordered simulation-based random variates $Z_1, \ldots, Z_M$ by $Z_{(1)} \geq Z_{(2)} \geq \cdots \geq Z_{(M)}$ and the corresponding parameter values by $\theta_{(1)}, \ldots, \theta_{(M)}$. In order to obtain an approximate lower bound on the Monte Carlo standard error for parameter estimator derived from pseudo-marginal MCMC, we consider the case where the second largest random error $\sigma Z_{(2)}$ is obtained at $\theta_{MESLE}$—that is, we assume $\theta_{(2)} = \theta_{MESLE}$. The proposal $\theta_{(1)}$ will be accepted with probability one, provided that

$$\mu(\theta_{(1)}) + \sigma Z_{(1)} \geq \mu(\theta_{(2)}) + \sigma Z_{(2)},$$

or

$$Z_{(1)} - Z_{(2)} \geq \sigma^{-1}\{\mu(\theta_{(2)}) - \mu(\theta_{(1)}\} = \sigma^{-1}(\theta_{(1)} - \theta_{(2)})^\top c(\theta_{(1)} - \theta_{(2)}). \tag{S33}$$

Denoting the cdf for the standard normal distribution by $\Phi(x)$, we use the result

$$1 - \Phi(x) = \frac{1}{\sqrt{2\pi}}\left(\frac{1}{x} + O\left(\frac{1}{x^3}\right)\right)e^{-x^2/2} \tag{S34}$$

[1]. For $0 < \epsilon < 1$, denote by $x_\epsilon$ the value satisfying $1 - \Phi(x_\epsilon) = \epsilon$. We approximate $Z_{(1)}$ by $x_{1/M}$ and $Z_{(2)}$ by $x_{2/M}$. Using (S34), we can approximate

$$Z_{(1)} \approx x_{1/M} \approx \sqrt{W\left(\frac{M^2}{2\pi}\right)}, \quad Z_{(2)} \approx x_{2/M} \approx \sqrt{W\left(\frac{M^2}{8\pi}\right)}$$

where $W(t)$ is the Lambert $W$ function satisfying $W(t)\exp\{W(t)\} = t$ [13]. Since $W(t) = \log t - \log\log t + O(\log\log t/\log t)$ for large $t$ [8], we approximate

$$\begin{aligned} Z_{(1)} - Z_{(2)} &\approx \sqrt{W\left(\frac{M^2}{2\pi}\right)} - \sqrt{W\left(\frac{M^2}{8\pi}\right)} \approx \sqrt{2\log M - \log 2\pi} - \sqrt{2\log M - \log 8\pi} \\ &\approx \sqrt{2\log M}\left\{1 - \frac{\log 2\pi}{4\log M} - \left(1 - \frac{\log 8\pi}{4\log M}\right)\right\} = O((\log M)^{-1/2}). \end{aligned}$$

Hence, from (S33) we have

$$\|\theta_{(1)} - \theta_{MESLE}\| = \|c\|^{-1/2}\sigma^{1/2}(\log(M))^{-1/4} = \emptyset((\log M)^{-1/4}).$$

## S8.2 Justification of the fact that the variance of Equation 35 scales as $\emptyset(k/\log J)$

When the likelihood is estimated using the particle filter with $J$ particles, Equation S8.2 in Section 6 shows that $\ell_i^S$ can be approximated as

$$\ell_i^S \approx \max_{j \in 1\,:\,J} \log g_i(y_i|X_i^j) - \log J,$$

provided that the dimension $k$ of $y_i$ is at least moderately large. In this section, we numerically demonstrate that the variance of $\ell_i^S$ scales as $\emptyset(k/\log J)$, given that $\log g_i(y_i|X_i^j)$ is approximately normally distributed. This normality assumption is reasonable if $\log g_i(y_i|X_i^j)$ is given by the sum of the log measurement densities for the $k$ components of $y_i$.

Figure S-10 shows the inverse of the variance of $\max_{j\in 1\,:\,J} Z_j$, where $Z_j$ are iid standard normal random variables. This result shows that $\text{Var}(\max_{j\in 1\,:\,J} Z_j)$ scales inversely proportional to $\log J$. Thus, given that the variance of $\log g_i(y_i|X_i^j)$ increases linearly with $k$, the variance of $\ell_i^S$ scales as $\emptyset(k/\log J)$.

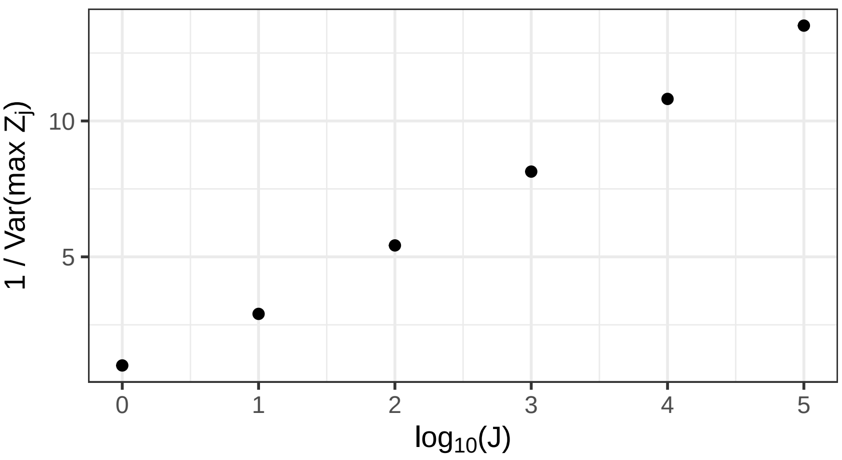


Figure S-10: The inverse of the variance of $\max_{j\in 1:J} Z_j$ for $J$ varying across 1, 10, $10^2$, $10^3$, $10^4$, and $10^5$.

# S9 Additional information on Section 7

## S9.1 Additional information on Section 7.1

Section 7.1 introduces an algorithm that automatically adjusts the weights of the simulation points for bias reduction. This algorithm aims balance using as many points as possible for efficient parameter estimation with narrowing the range of parameter values used for simulation to ensure that quadratic approximation introduces little bias. The weights are adjusted by multiplying a discount factor given by

$$\exp\left(-\frac{q_2(\hat{\theta}_{MESLE}) - q_2(\theta)}{g}\right)$$

for parameter value $\theta$. However, the value of $g$ can sometimes decrease to a point where there are insufficient effective number of simulation points for parameter estimation. In order for cubic regression to be numerically stable, the effective sample size (ESS) should satisfy

$$\text{ESS} := \frac{(\sum_{m=1}^{M} w_m^{adj})^2}{\sum_{m=1}^{M} {w_m^{adj}}^2} \gtrsim \frac{(d+1)(d+2)(d+3)}{6}, \tag{S35}$$

where $(d+1)(d+2)(d+3)/6$ is the total number of scalar parameters being estimated in cubic regression ($d$ is the dimension of the parameter vector). If this condition is not satisfied, $g$ is increased to a level where the ESS grows above the required threshold. Note that the effective sample size defined in (S35) differs from the ESS defined in (33) in Section 6 to compare the efficiency of our method with that of pseudo-marginal MCMC. Algorithm 1 summarizes the modified procedure taking into account the ESS for weight adjustments.

In the `sbim` package, adding the option `autoAdjust=TRUE` in the functions `ht`() and `ci`() enables automatic weight adjustments as described in Algorithm 1.

## S9.2 Additional information on Section 7.2

Section 7.2 introduces an algorithm that proposes the next simulation point by minimizing the Monte Carlo variation in parameter estimation (Algorithm 5). Suppose that a new simulation is carried out at $\theta_{M+1}$ and that $\hat{A}_{M+1}$ denotes the coefficients of the new quadratic polynomial fitted to $(\theta_m, \ell^S(\theta_m))$ with weights $w_m^{adj}$, $m \in 1\!:\!M+1$, where the adjusted weight for the new point is given by

$$w_{M+1}^{adj} = w_{M+1} \cdot \exp\left(-\frac{(\hat{b}^\top \hat{\theta}_{MESLE} + \hat{\theta}_{MESLE}^\top \hat{c}\hat{\theta}_{MESLE}) - (\hat{b}^\top \theta_{M+1} + \theta_{M+1}^\top \hat{c}\theta_{M+1})}{g}\right).$$

**Algorithm 1** Automatic weight adjustments for bias reduction (with the consideration of effective sample size)

Fit a quadratic polynomial to $(\theta_m, \ell^S(\theta_m))$ with weights $w_m$, $m \in 1:M$, to obtain a first-stage quadratic approximation $q_2(\theta) = \hat{a} + \hat{b}^\top \theta + \theta^\top \hat{c} \theta$<br>
Let $\hat{\theta}_{MESLE} = -\frac{1}{2}\hat{c}^{-1}\hat{b} = \arg\max_\theta q_2(\theta)$ be the estimated MESLE<br>
Let $g \leftarrow \infty$<br>
Let ExitUponSufficientESS $\leftarrow$ FALSE<br>
**loop**<br>
    Weight adjustments: $w_m^{adj} = w_m \cdot \exp(-\{q_2(\hat{\theta}_{MESLE}) - q_2(\theta_m)\}/g)$<br>
    Compute effective sample size: $\text{ESS} = (\sum_{m=1}^{M} w_m^{adj})^2 / (\sum_{m=1}^{M} {w_m^{adj}}^2)$<br>
    **if** $\text{ESS} < (d+1)(d+2)(d+3)/6$ **then** ▷ numerically instable cubic regression<br>
        Let ExitUponSufficientESS $\leftarrow$ TRUE<br>
        Let $g \leftarrow 1.5g$<br>
        Go to the next iteration<br>
    **end if**<br>
    **if** ExitUponSufficientESS **then**<br>
        Break from loop<br>
    **end if**<br>
    Update $q_2$ and $\hat{\theta}_{MESLE}$ using the adjusted weights<br>
    Fit a cubic polynomial to $(\theta_m, \ell^S(\theta_m))$ with weights $w_m^{adj}$, $m \in 1:M$<br>
    Let $p_{\text{cubic}}$ be the p-value for the significance of the cubic term<br>
    **if** $p_{\text{cubic}} < 0.01$ **then** ▷ cubic term is significant, decrease $g$<br>
        **if** $g = \infty$ **then**<br>
            Let $g \leftarrow q_2(\hat{\theta}_{MESLE}) - \min_{m \in 1:M} q_2(\theta_m)$<br>
        **else**<br>
            Let $g \leftarrow g/1.8$<br>
        **end if**<br>
    **else if** $p_{\text{cubic}} > 0.3$ **then** ▷ cubic term is not significant, increase $g$ for efficiency<br>
        Let $g \leftarrow 1.3 \cdot g$<br>
    **else**<br>
        Break from loop<br>
    **end if**<br>
**end loop**

The value of $g$ is determined using Algorithm 4. The variance of these updated set of coefficients is given by

$$\text{Var}(\hat{A}_{M+1}) = \sigma^2 \{ {\theta_{1:M}^{0:2}}^\top W^{adj} \theta_{1:M}^{0:2} + w_{M+1}^{adj} \theta_{M+1}^{0:2} {\theta_{M+1}^{0:2}}^\top \}^{-1}.$$

After the addition of the $(M+1)$th simulation point, the Monte Carlo variance of the estimated MESLE is approximated by $\sigma^2 V_{M+1}(\theta_{M+1})$, where

$$V_{M+1}(\theta_{M+1}) := \left( \frac{\partial \hat{\theta}_{MESLE}}{\partial \hat{A}} \right) \{ {\theta_{1:M}^{0:2}}^\top W^{adj} \theta_{1:M}^{0:2} + w_{M+1}^{adj} \theta_{M+1}^{0:2} {\theta_{M+1}^{0:2}}^\top \}^{-1} \left( \frac{\partial \hat{\theta}_{MESLE}}{\partial \hat{A}} \right)^\top.$$

Since

$$\frac{\partial \hat{\theta}_{MESLE}}{\partial \hat{A}} = -\frac{1}{2} \frac{\partial \hat{c}^{-1} \hat{b}}{\partial (\hat{a}, \hat{b}, \text{vech}(\hat{c}))}$$

only depends on $\hat{b}$ and $\hat{c}$, the matrix $V_{M+1}$ depends on $\theta_{M+1}$ only through the middle term. In order to quantify the total amount of Monte Carlo variation in the parameter estimate, we consider a scaled total variation (STV) measure defined by

$$\text{STV}(\theta_{M+1}) := \text{Tr}\{ -\hat{c}^{-1} V_{M+1}(\theta_{M+1}) \}$$

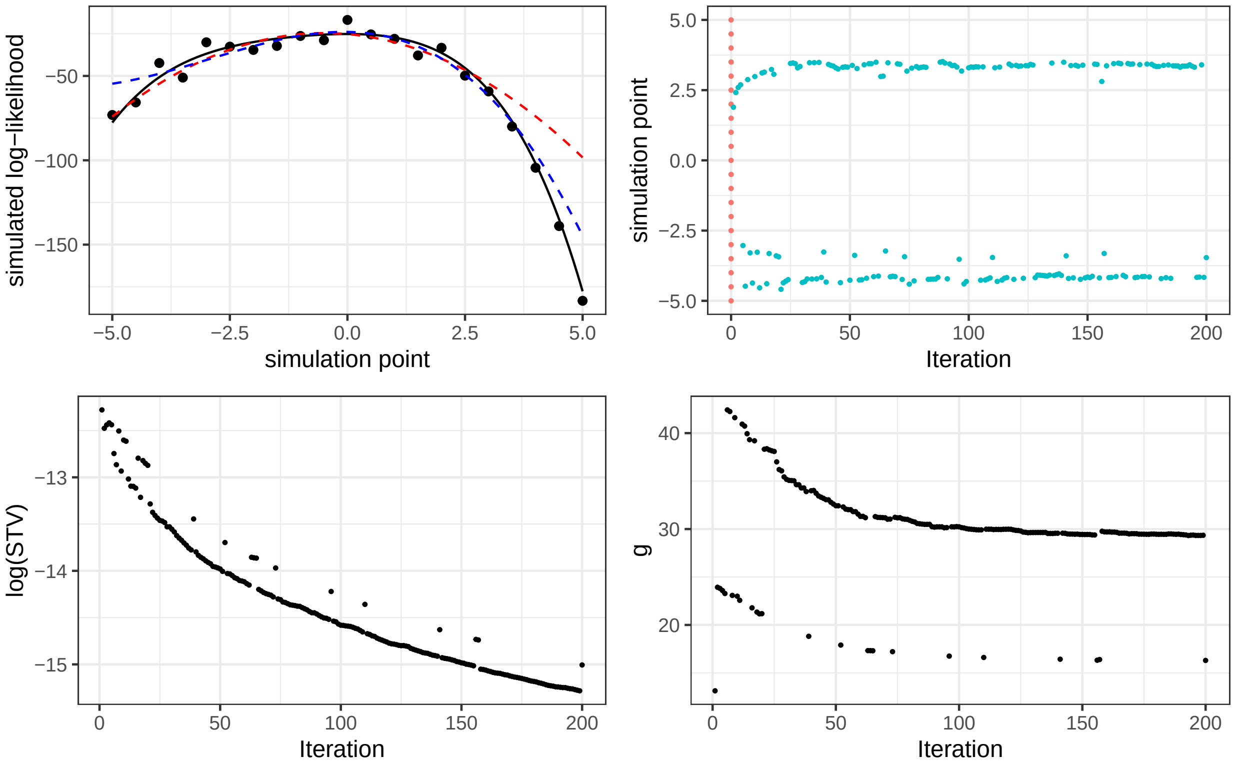


Figure S-11: Top left: Simulated log-likelihoods for initial points for Example S7. The black curve indicates the expected simulation log-likelihood function, $\mu(\theta)$. The red and blue dashed curves show the fitted quadratic and cubic polynomials, respectively. Top right: Simulation points iteratively proposed by Algorithm 5. The initial simulation points are indicated by red dots. Bottom left: Logarithms of scaled total variation (STV) over iterations. Bottom right: Tuned values of $g$ over iterations.

where $-\hat{c}$ is the curvature of the fitted quadratic function before the addition of the new simulation point. The multiplication by $-\hat{c}^{-1}$ ensures that the estimation scales of the parameter components are taken into account when summing the Monte Carlo variances.

The optimization of STV can be rapidly performed using the Broyden–Fletcher–Goldfarb–Shanno (BFGS) algorithm, which uses the graidents of the objective function [7]. Writing

$$\Omega = {\theta^{0:2}_{1:M}}^\top W^{adj} \theta^{0:2}_{1:M} + w^{adj}_{M+1} \theta^{0:2}_{M+1} {\theta^{0:2}_{M+1}}^\top,$$

we can express the derivative of STV with respect to the $i$-th component of $\theta_{M+1}$ by

$$\frac{\partial \text{STV}}{\partial \theta_{M+1,(i)}} = \text{Tr}\left\{ \hat{c}^{-1} \left( \frac{\partial \hat{\theta}_{MESLE}}{\partial \hat{A}} \right) \Omega^{-1} \frac{\partial \Omega}{\partial \theta_{M+1,(i)}} \Omega^{-1} \left( \frac{\partial \hat{\theta}_{MESLE}}{\partial \hat{A}} \right)^\top \right\}$$

where

$$\frac{\partial \Omega}{\partial \theta_{M+1,(i)}} = w^{adj}_{M+1} g^{-1} (\hat{b} + 2\hat{c}\theta_{M+1})_{(i)} \theta^{0:2}_{M+1} {\theta^{0:2}_{M+1}}^\top + w^{adj}_{M+1} \frac{\partial \theta^{0:2}_{M+1}}{\partial \theta_{M+1,(i)}} {\theta^{0:2}_{M+1}}^\top + w^{adj}_{M+1} \theta^{0:2}_{M+1} {\frac{\partial \theta^{0:2}_{M+1}}{\partial \theta_{M+1,(i)}}}^\top.$$

**Example S7.** We generate simulated log-likelihoods from an artificial metamodel

$$\ell^S(\theta) = -(\theta - 0.2)^2 + \min(4, 0.2 \times \theta^3) - 0.1 \times (\theta + 1)^4 + \mathcal{N}(0, \sigma^2), \quad \theta \in \mathbb{R}$$

with $\sigma = 5$. Initially, simulations are carried out regular intervals of 0.5 over the range $[-5, 5]$.

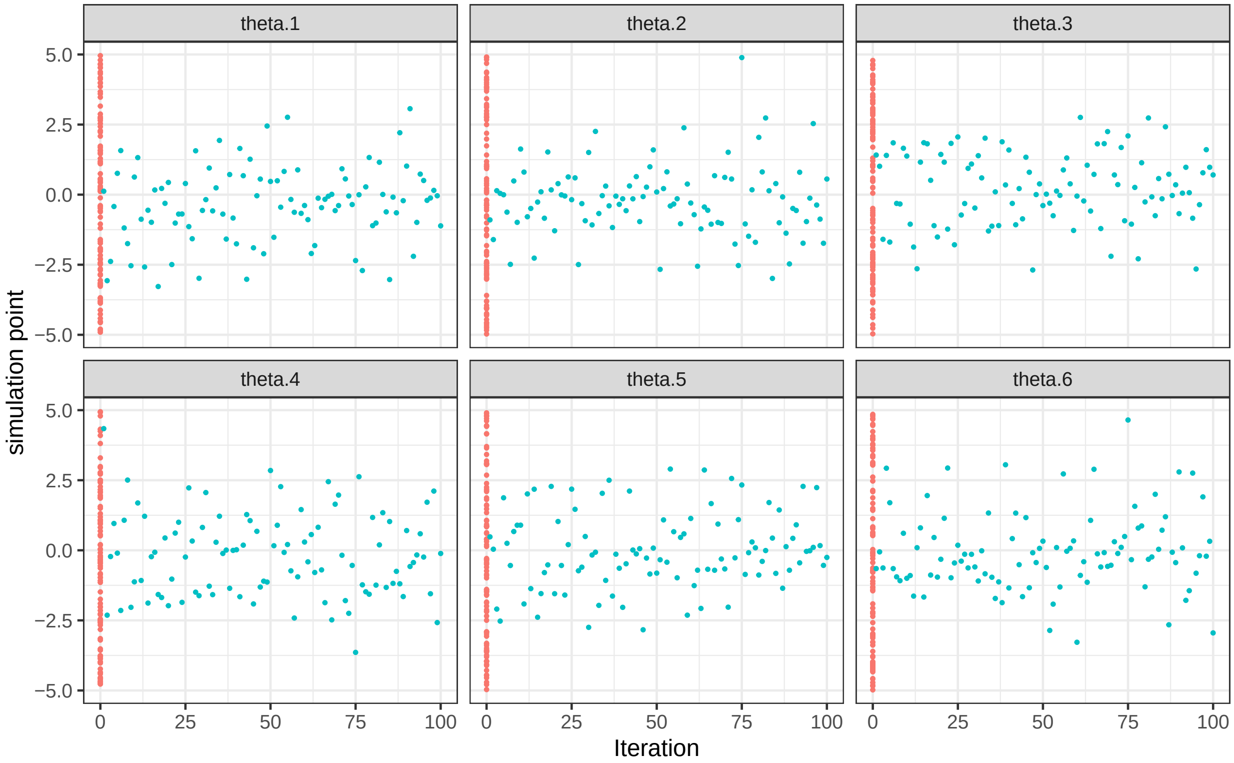


Figure S-12: Proposed simulation points for each of the $d = 6$ components for Example S8 using Algorithm 5. Red dots indicate the initial simulation points.

The simulated log-likelihoods for these initial points are shown in the top left plot of Figure S-11. The quadratic approximation (red dashed curve) deviates significantly from the cubic approximation (blue dashed curve) for $|\theta| \gtrsim 3$. The top right plot of Figure S-11 displays the proposed simulation points after Algorithm 5 is applied iteratively two hundred times. The proposed points alternate between two values, approximately -3 and 3. These results suggest that near-optimal points tend to be positioned as far as possible from the estimated MESLE while still ensuring sufficient accuracy in the quadratic approximation. Optimization of log(STV) was carried out using the automatically tuned value for $g$. However, for comparison across iterations, the bottom left plot of Figure S-11 shows log(STV) values evaluated at the proposed points using a fixed value of $g = 20$. These STV values generally decrease, indicating that the algorithm effectively reduces uncertainty in parameter estimation. Occasionally, STV takes a relative large values, which is due to the small tuned values for $g$ in those instances. The tuned values of $g$ are shown in the bottom right panel of Figure S-11. The fact that $g$ consistently drops suggests that as more simulation points are added, the cubic term becomes increasingly significant. Consequently, to preserve the fidelity of the quadratic approximation, the effective range of parameter values for inference shrinks.

We next considered a metamodel with a six-dimensional parameter space.

**Example S8.** Simulated log-likelihoods are generated from a metamodel

$$\ell^S(\theta) = -(\theta - \theta_0)^\top c(\theta - \theta_0) - 0.1 \times \sum_{i=1}^{6} \theta_{(i)}^4 + \mathcal{N}(0, \sigma^2).$$

Here $\theta_0$ is a random draw from $\mathcal{N}(0, 0.5^2 I_6)$, $c = U\Lambda U^\top$ where $U$ is a random draw from $SO(6)$ and $\Lambda$ is a diagonal matrix with diagonal entries independently drawn from Uniform(0,1), and $\sigma = 5$. Simulated log-likelihoods are initially obtained at one hundred randomly selected points $\theta_m$ with $\theta_{m,(i)} \overset{iid}{\sim}$ Uniform$(-5, 5)$. Subsequent simulation points are proposed using Algorithm 5 with fixed weight adjustment parameter $g = 20$.

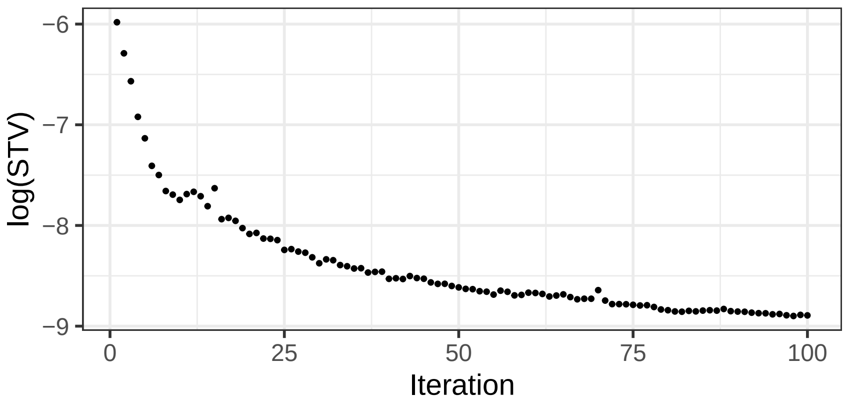


Figure S-13: Logarithms of STV at the proposed points for Example S8.

Figure S-12 shows the iteratively proposed simulation points. At each iteration, the optimization started from a randomly selected point, with each entry independently drawn from Uniform$(-5, 5)$. All six entries of the proposed points approximately fall between -2.5 and 2.5. We repeated this experiment using starting points whose entries were randomly drawn from Uniform$(-1, 1)$. The proposed points exhibited the same pattern, with a similar range of [-2.5, 2.5] (figure not shown). These results suggest that the simulation points are the minimizers of $\log(STV)$ and are largely independent of the initial values used for optimization. Figure S-13 shows the $\log(STV)$ values at the proposed points. The decreasing values of $\log(STV)$ indicate that Algorithm 5 successfully selectes points for efficient parameter estimation.

# Supplementary References


[1] M. Abramowitz and I. A. Stegun. *Handbook of Mathematical Functions with Formulas, Graphs, and Mathematical Tables. National Bureau of Standards Applied Mathematics Series 55. Tenth Printing.* National Bureau of Standards (DOC), Washington, D.C., 1972.

[2] A. Agresti. *Foundations of linear and generalized linear models.* John Wiley & Sons, 2015.

[3] L. V. Ahlfors. *Complex analysis.* McGraw-Hill, second edition, 1966.

[4] J. Bérard, P. Del Moral, and A. Doucet. A lognormal central limit theorem for particle approximations of normalizing constants. *Electron. J. Probab*, 19(94):1–28, 2014.

[5] K. L. Chung. *A course in probability theory.* Academic press, third edition, 2001.

[6] P. Doukhan, P. Massart, and E. Rio. The functional central limit theorem for strongly mixing processes. *Ann. Inst. Henri Poincar ´e Probab. Stat.*, 30(1):63–82, 1994.

[7] R. Fletcher. *Practical methods of optimization.* John Wiley & Sons, second edition, 1987.

[8] A. Hoorfar and M. Hassani. Inequalities on the lambert w function and hyperpower function. *J. Inequal. Pure and Appl. Math*, 9(2):5–9, 2008.

[9] M. Kendall and A. Stuart. *The advanced theory of statistics. Vol. 1: Distribution theory.* MacMillan Publishing, New York, 4th edition, 1977.

[10] T.-T. Lu and S.-H. Shiou. Inverses of 2× 2 block matrices. *Comput. Math. Appl.*, 43(1-2):119–129, 2002.

[11] E. Lukacs. *Characteristic functions, Griffin's Statistical Monographs& Courses, No. 5.* Griffin: London, 1960.

[12] K. P. Murphy. *Machine learning: a probabilistic perspective.* MIT press, 2012.

[13] E. W. Weisstein. Lambert w-function. From MathWorld—A Wolfram Web Resource, 2024. Last visited on 5/21/2024.

[14] M. A. Woodbury. Inverting modified matrices. Statistical Research Group, Memo. Rep., no. 42, Princeton University, Princeton, N. J., 1950.

[15] A. Zellner. Bayesian and non-Bayesian analysis of the regression model with multivariate student-t error terms. *J. Amer. Statist. Assoc.*, 71(354):400–405, 1976.
